# Supplementary material for: Relaxing Hardware Requirements for Surface Code Circuits using Time-dynamics
Source: arXiv:2302.02192 ancillary file (2023-09-14)
Supplement: Supplementary file 1 [file supplementary_figures.pdf]

# Supplementary Figures for “Relaxing Hardware Requirements for Surface Code Circuits using Time-dynamics”

Matt McEwen[1], Dave Bacon[2], and Craig Gidney[1]

[1]Google Quantum AI, Santa Barbara, California 93117, USA

[2]Google Quantum AI, Seattle, Washington 98103, USA

February 3, 2023

Matt McEwen: mmcewen@google.com

Dave Bacon: dabacon@google.com

Craig Gidney: craig.gidney@gmail.com

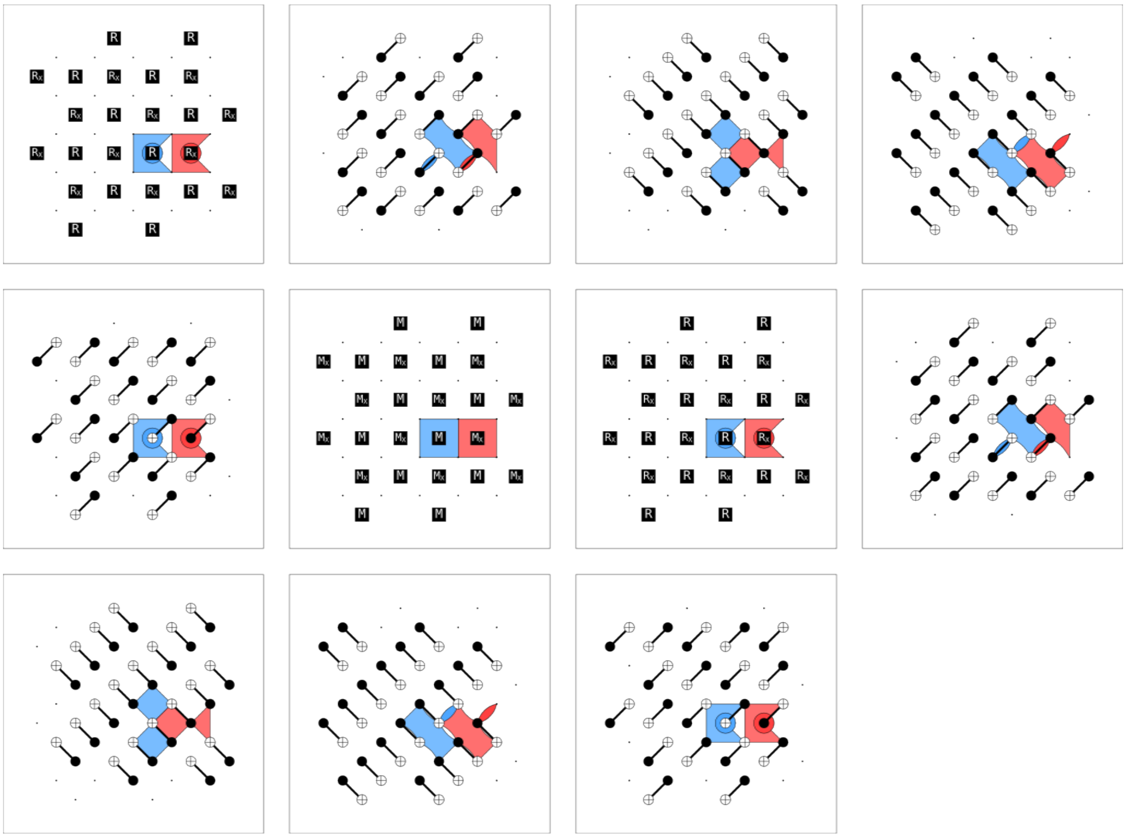

Figure 1: Circuit schedule for "4-CX" circuits. Colored regions are elements of the instantaneous stabilizer group formed by slicing the detecting regions of a few representative detectors immediately after the displayed gate layer. Red regions are X stabilizers, blue regions are Z stabilizers, green regions are Y stabilizers, and gray regions with colored corners are mixed basis stabilizers.

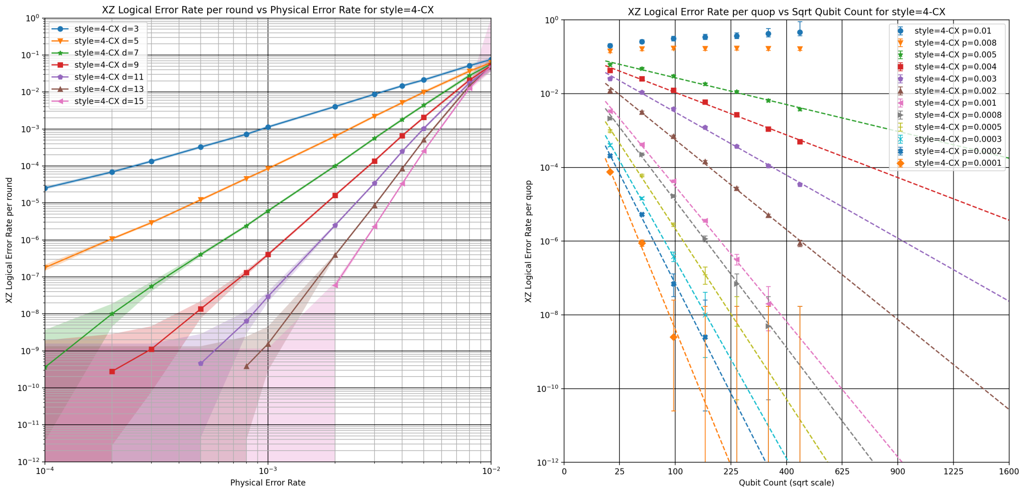


Figure 2: Threshold diagram and line fit diagram for "4-CX" circuits. Highlighted regions cover hypotheses with likelihoods within a factor of 1000 of the maximum likelihood hypothesis. Dashed lines are least squares fits projecting the number of qubits needed to reach a target error rate.

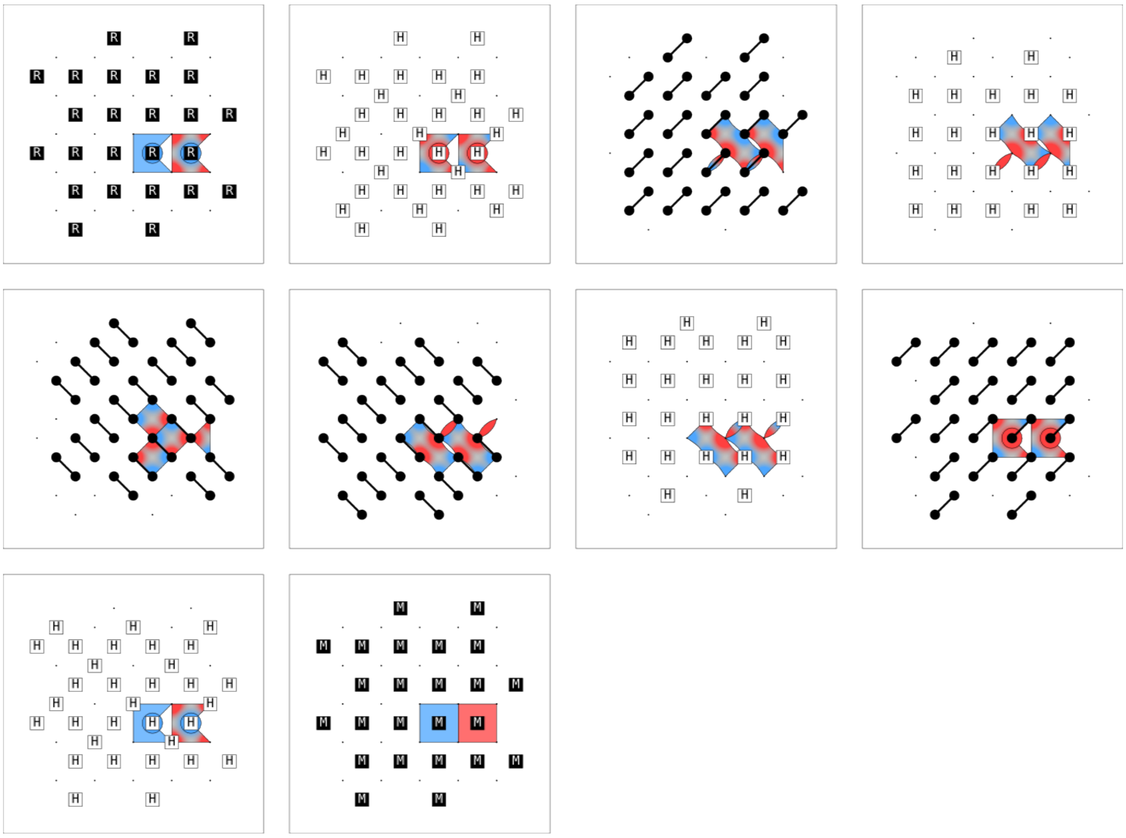

Figure 3: Circuit schedule for “4-CZ” circuits. Colored regions are elements of the instantaneous stabilizer group formed by slicing the detecting regions of a few representative detectors immediately after the displayed gate layer. Red regions are X stabilizers, blue regions are Z stabilizers, green regions are Y stabilizers, and gray regions with colored corners are mixed basis stabilizers.

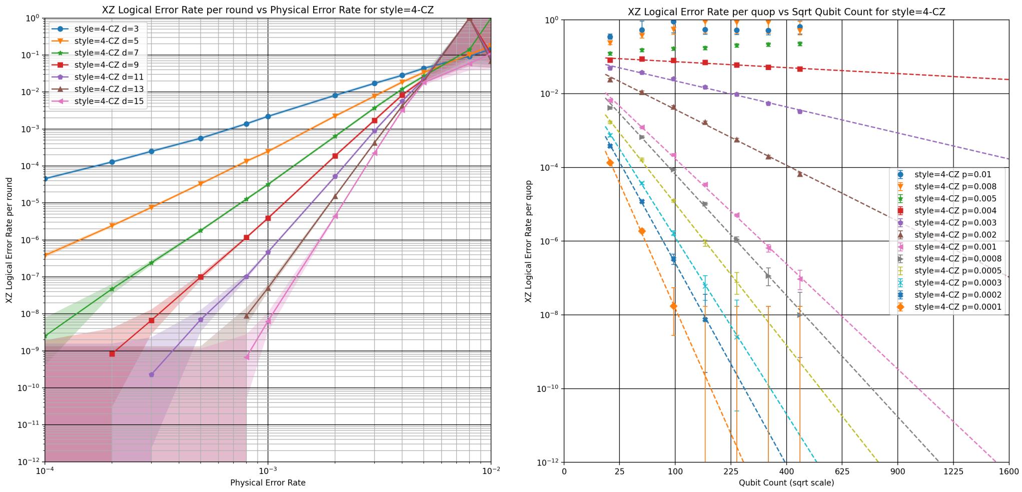


Figure 4: Threshold diagram and line fit diagram for “4-CZ” circuits. Highlighted regions cover hypotheses with likelihoods within a factor of 1000 of the maximum likelihood hypothesis. Dashed lines are least squares fits projecting the number of qubits needed to reach a target error rate.

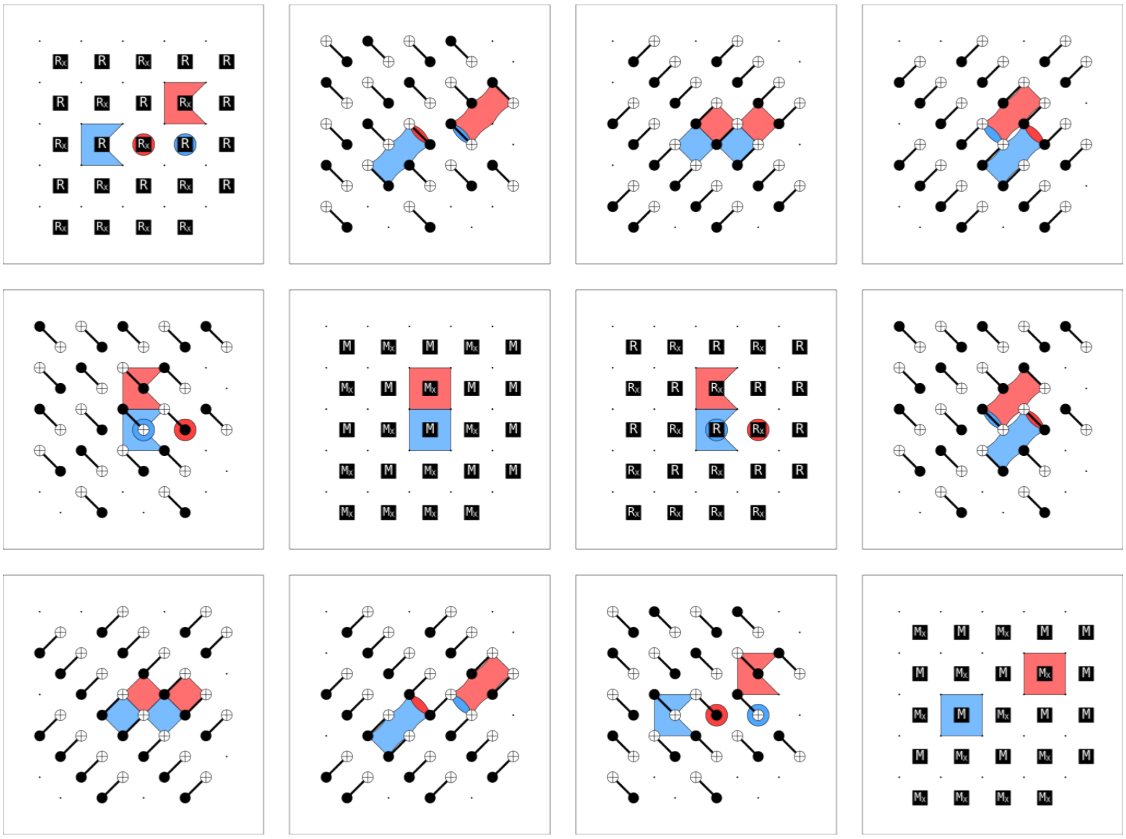

Figure 5: Circuit schedule for "3-CX" circuits. Colored regions are elements of the instantaneous stabilizer group formed by slicing the detecting regions of a few representative detectors immediately after the displayed gate layer. Red regions are X stabilizers, blue regions are Z stabilizers, green regions are Y stabilizers, and gray regions with colored corners are mixed basis stabilizers.

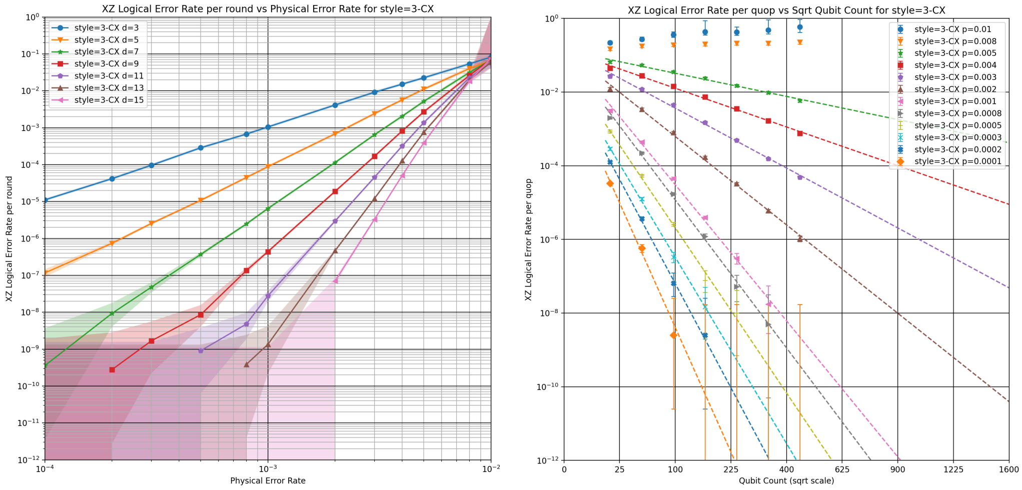


Figure 6: Threshold diagram and line fit diagram for "3-CX" circuits. Highlighted regions cover hypotheses with likelihoods within a factor of 1000 of the maximum likelihood hypothesis. Dashed lines are least squares fits projecting the number of qubits needed to reach a target error rate.

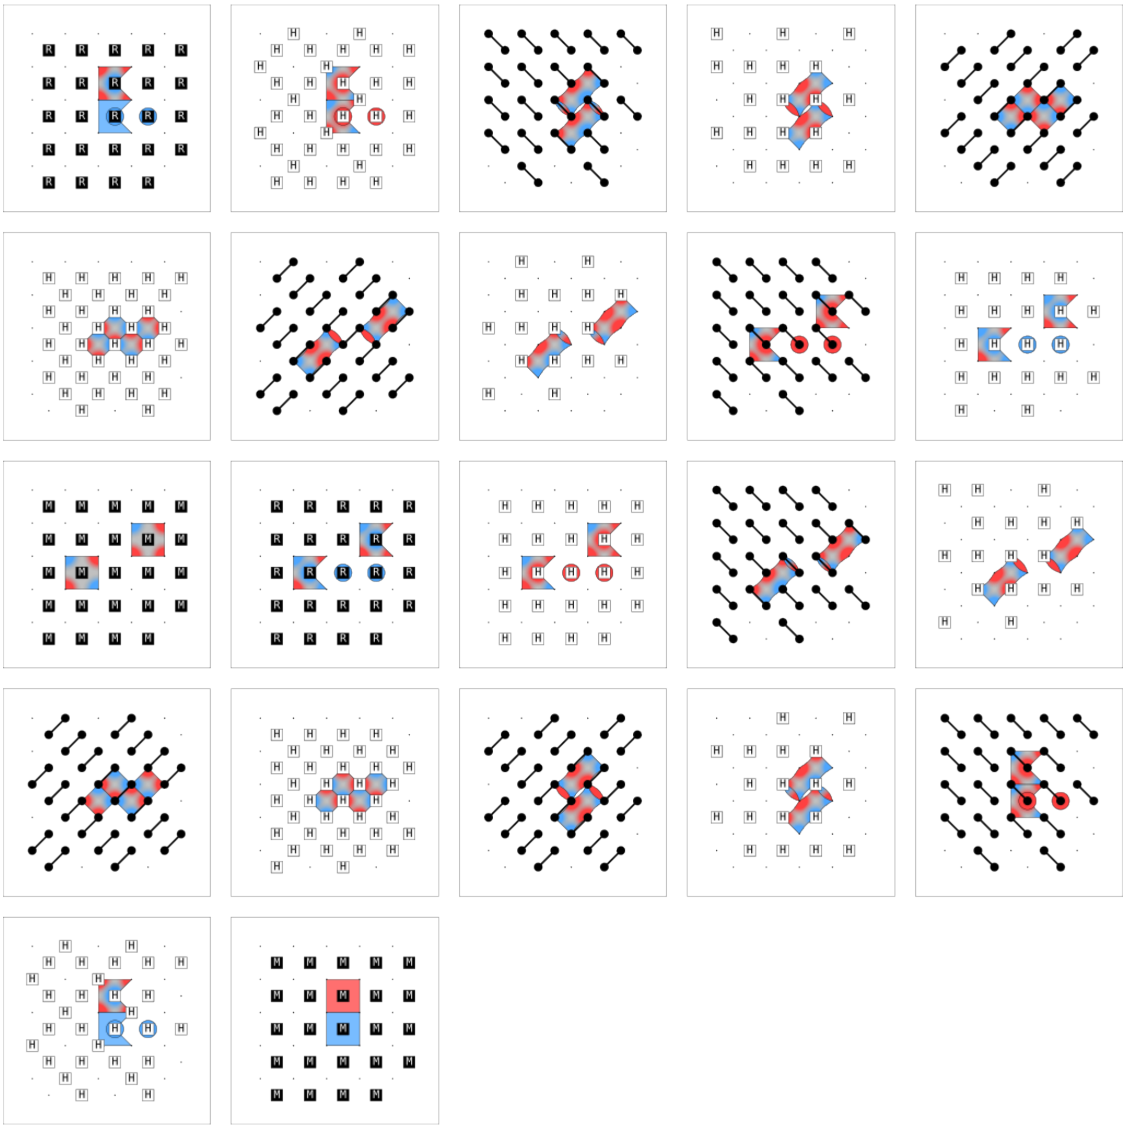

Figure 7: Circuit schedule for "3-CZ" circuits. Colored regions are elements of the instantaneous stabilizer group formed by slicing the detecting regions of a few representative detectors immediately after the displayed gate layer. Red regions are X stabilizers, blue regions are Z stabilizers, green regions are Y stabilizers, and gray regions with colored corners are mixed basis stabilizers.

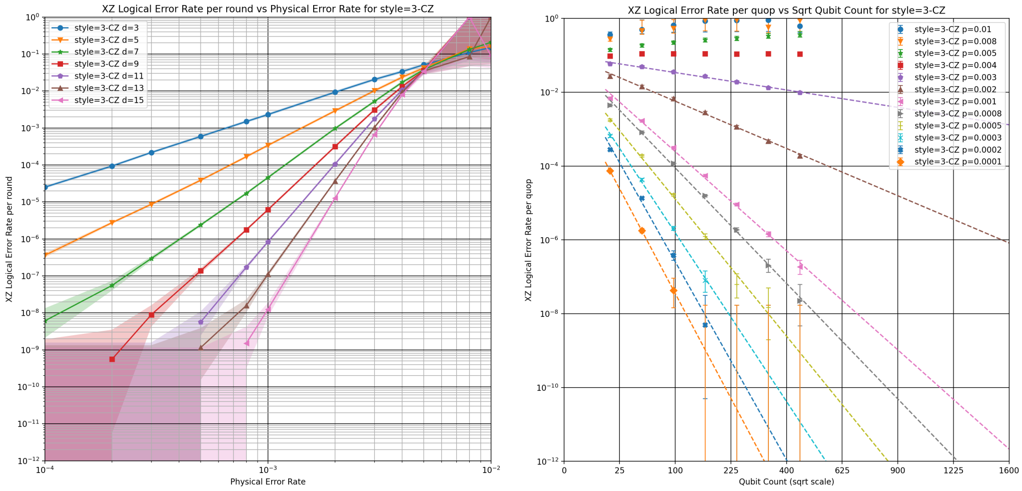


Figure 8: Threshold diagram and line fit diagram for “3-CZ” circuits. Highlighted regions cover hypotheses with likelihoods within a factor of 1000 of the maximum likelihood hypothesis. Dashed lines are least squares fits projecting the number of qubits needed to reach a target error rate.

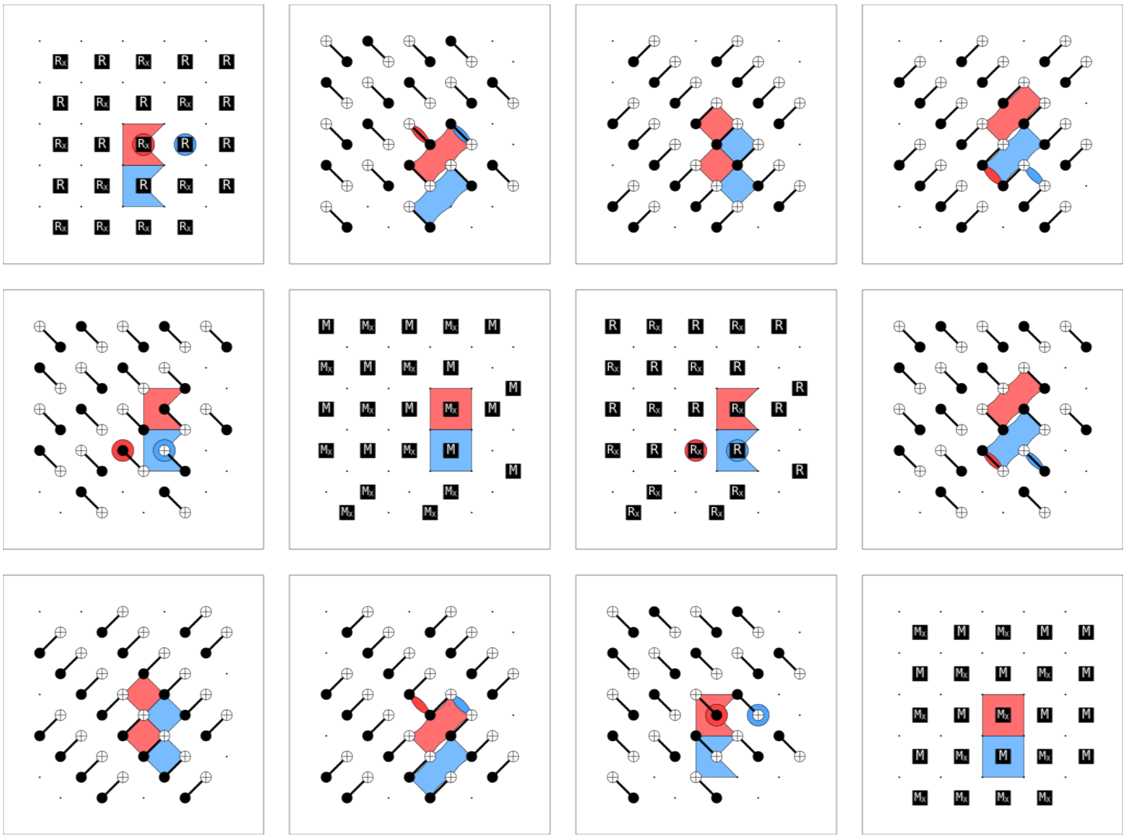

Figure 9: Circuit schedule for "3-CX-wiggle" circuits. Colored regions are elements of the instantaneous stabilizer group formed by slicing the detecting regions of a few representative detectors immediately after the displayed gate layer. Red regions are X stabilizers, blue regions are Z stabilizers, green regions are Y stabilizers, and gray regions with colored corners are mixed basis stabilizers.

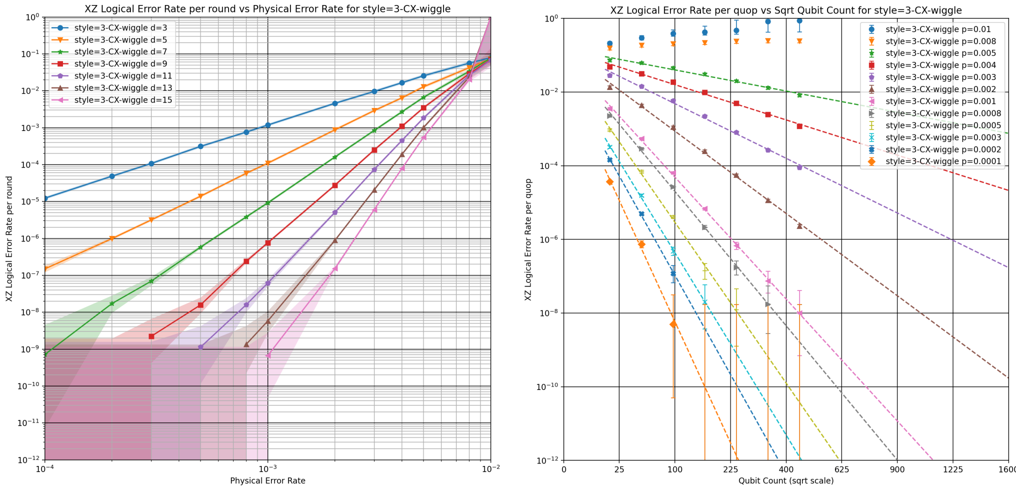


Figure 10: Threshold diagram and line fit diagram for "3-CX-wiggle" circuits. Highlighted regions cover hypotheses with likelihoods within a factor of 1000 of the maximum likelihood hypothesis. Dashed lines are least squares fits projecting the number of qubits needed to reach a target error rate.

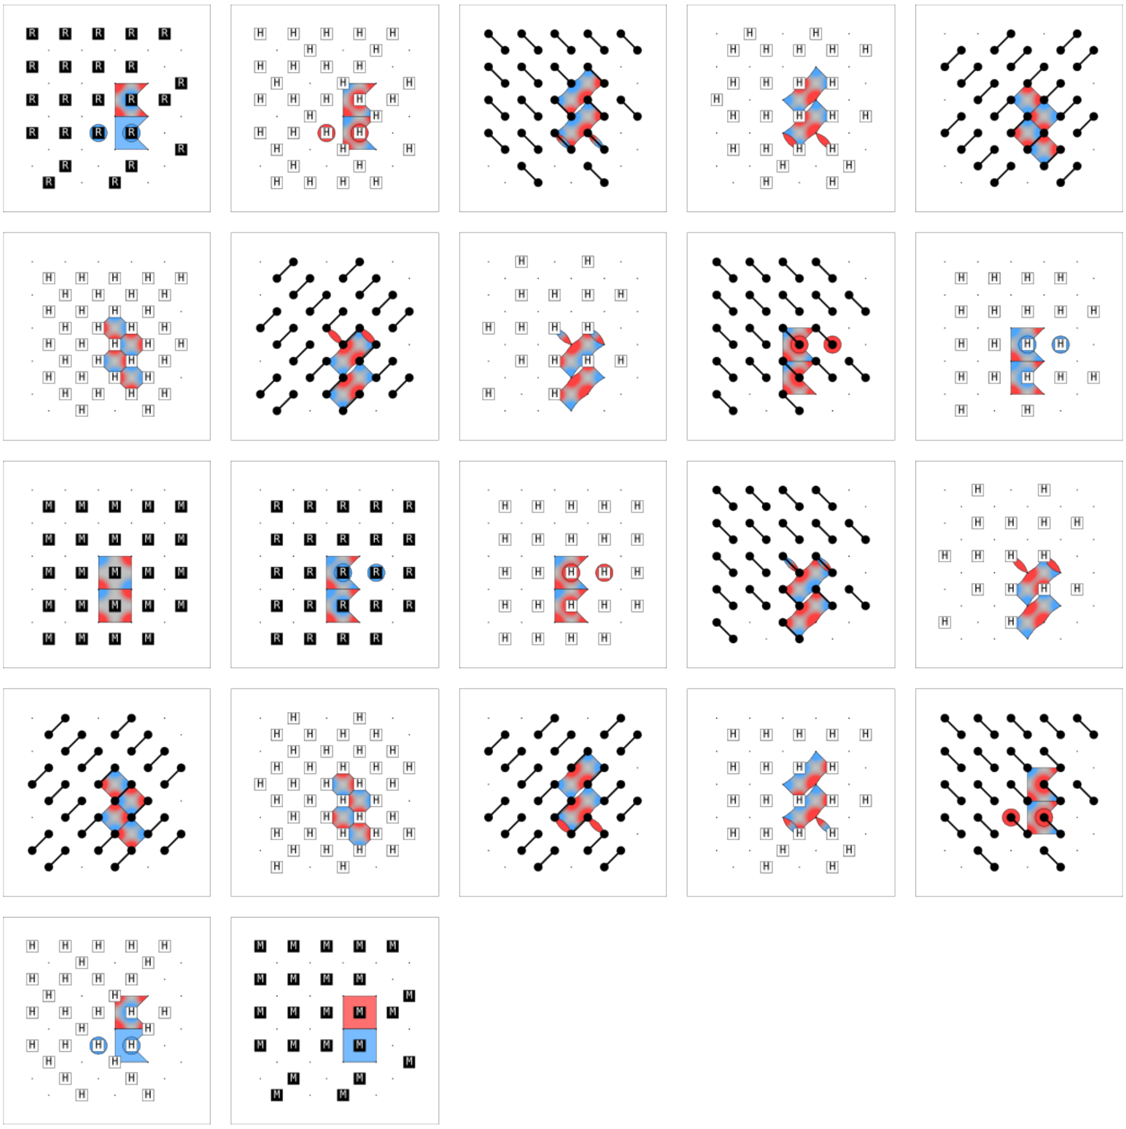

Figure 11: Circuit schedule for "3-CZ-wiggle" circuits. Colored regions are elements of the instantaneous stabilizer group formed by slicing the detecting regions of a few representative detectors immediately after the displayed gate layer. Red regions are X stabilizers, blue regions are Z stabilizers, green regions are Y stabilizers, and gray regions with colored corners are mixed basis stabilizers.

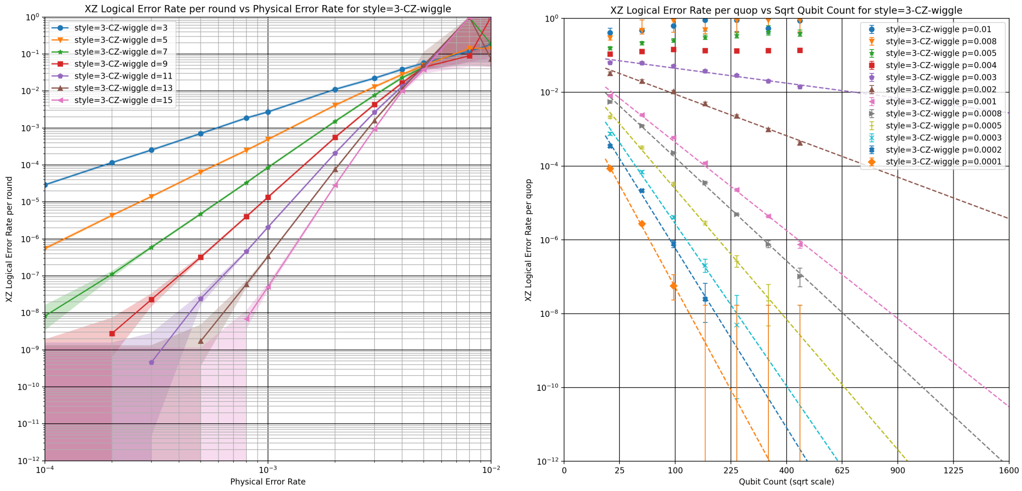


Figure 12: Threshold diagram and line fit diagram for “3-CZ-wiggle” circuits. Highlighted regions cover hypotheses with likelihoods within a factor of 1000 of the maximum likelihood hypothesis. Dashed lines are least squares fits projecting the number of qubits needed to reach a target error rate.

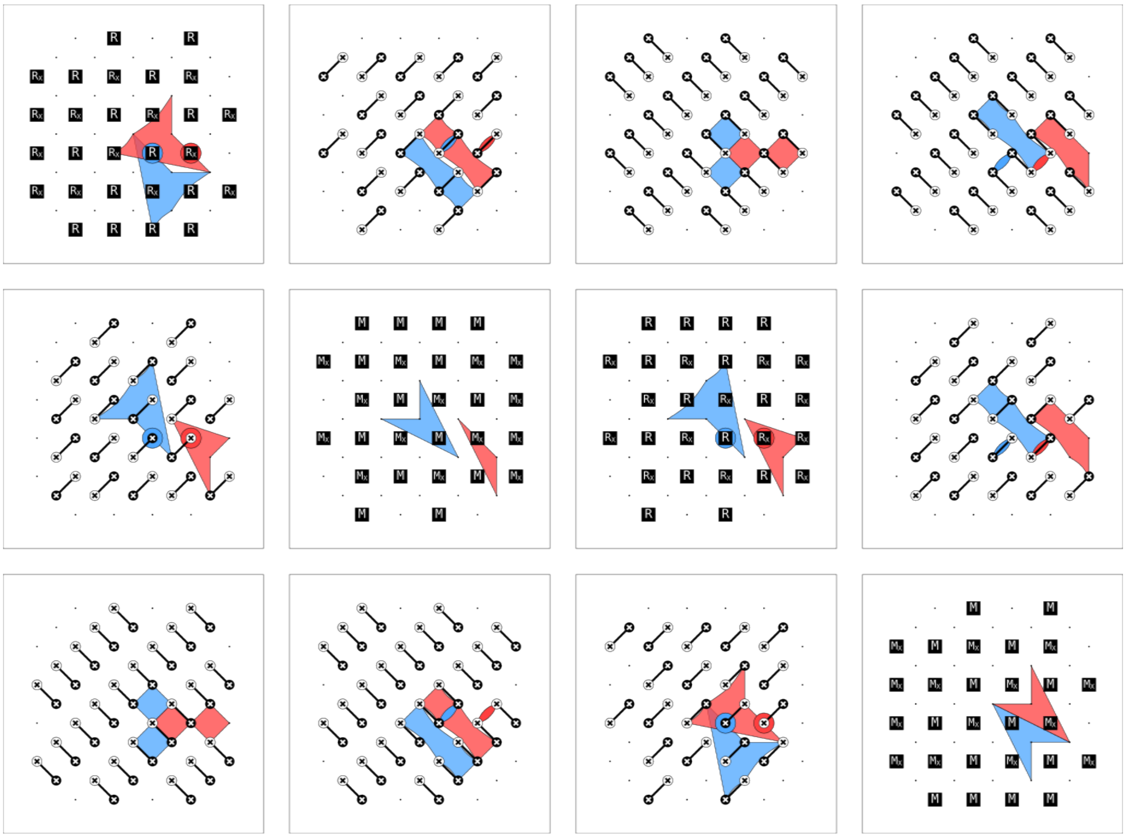

Figure 13: Circuit schedule for “4-CXSWAP” circuits. Colored regions are elements of the instantaneous stabilizer group formed by slicing the detecting regions of a few representative detectors immediately after the displayed gate layer. Red regions are X stabilizers, blue regions are Z stabilizers, green regions are Y stabilizers, and gray regions with colored corners are mixed basis stabilizers.

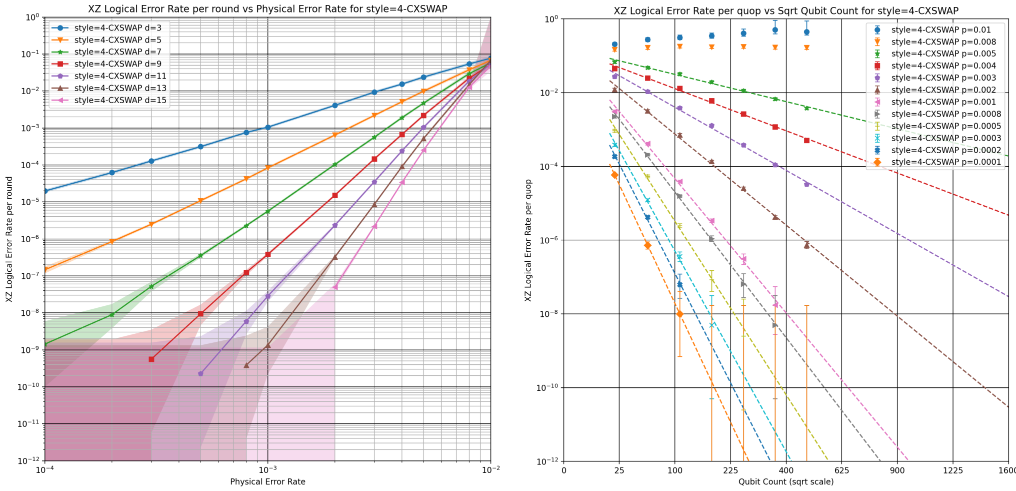


Figure 14: Threshold diagram and line fit diagram for “4-CXSWAP” circuits. Highlighted regions cover hypotheses with likelihoods within a factor of 1000 of the maximum likelihood hypothesis. Dashed lines are least squares fits projecting the number of qubits needed to reach a target error rate.

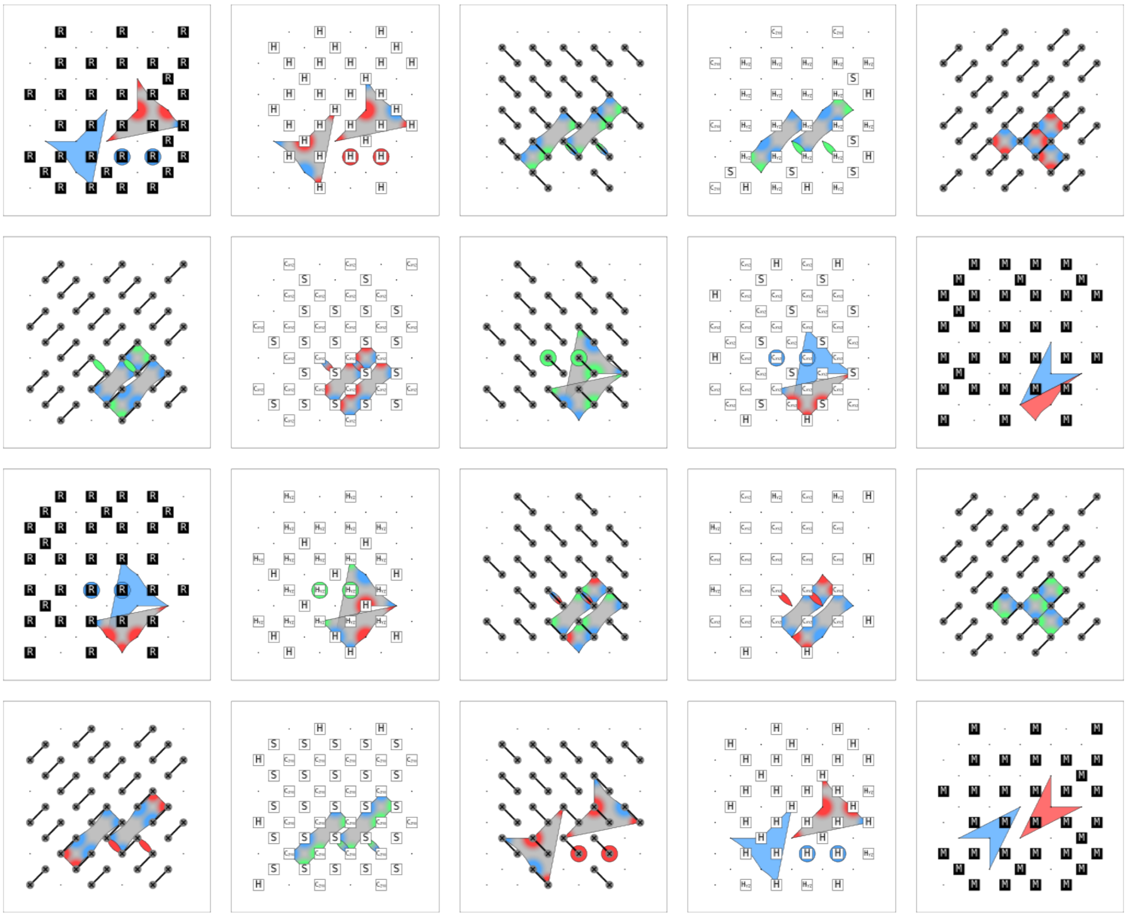

Figure 15: Circuit schedule for "4-ISWAP" circuits. Colored regions are elements of the instantaneous stabilizer group formed by slicing the detecting regions of a few representative detectors immediately after the displayed gate layer. Red regions are X stabilizers, blue regions are Z stabilizers, green regions are Y stabilizers, and gray regions with colored corners are mixed basis stabilizers.

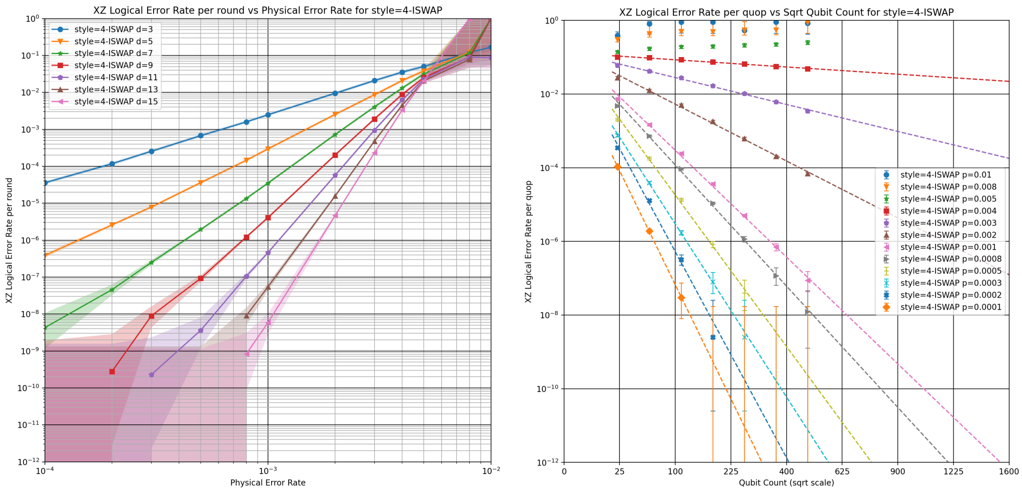


Figure 16: Threshold diagram and line fit diagram for "4-ISWAP" circuits. Highlighted regions cover hypotheses with likelihoods within a factor of 1000 of the maximum likelihood hypothesis. Dashed lines are least squares fits projecting the number of qubits needed to reach a target error rate.

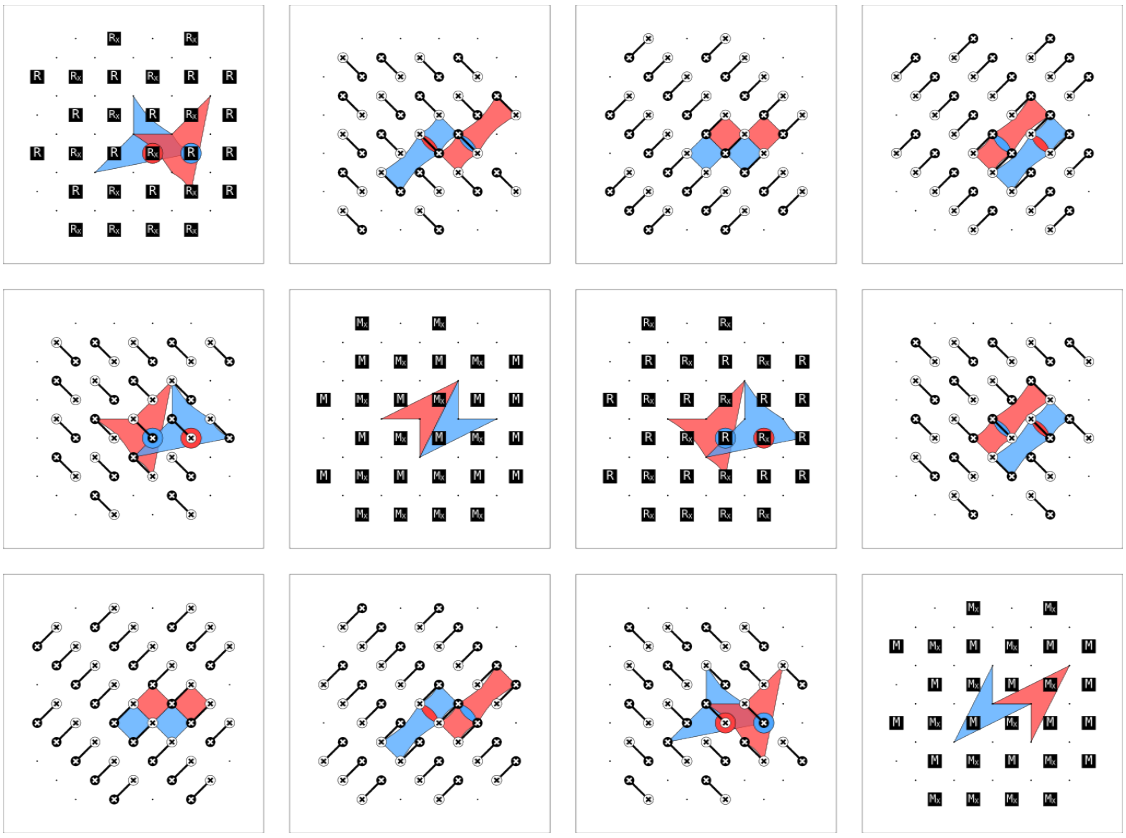

Figure 17: Circuit schedule for “3-CXSWAP” circuits. Colored regions are elements of the instantaneous stabilizer group formed by slicing the detecting regions of a few representative detectors immediately after the displayed gate layer. Red regions are X stabilizers, blue regions are Z stabilizers, green regions are Y stabilizers, and gray regions with colored corners are mixed basis stabilizers.

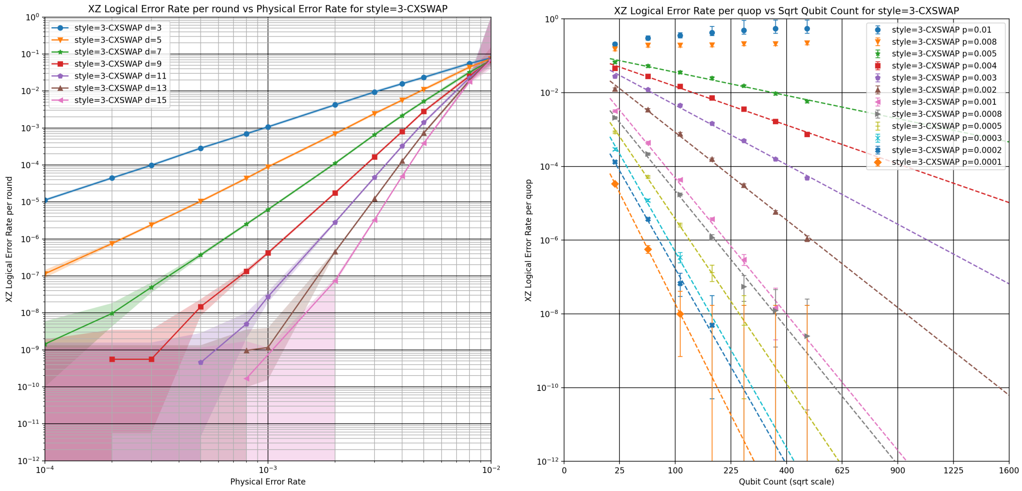


Figure 18: Threshold diagram and line fit diagram for “3-CXSWAP” circuits. Highlighted regions cover hypotheses with likelihoods within a factor of 1000 of the maximum likelihood hypothesis. Dashed lines are least squares fits projecting the number of qubits needed to reach a target error rate.

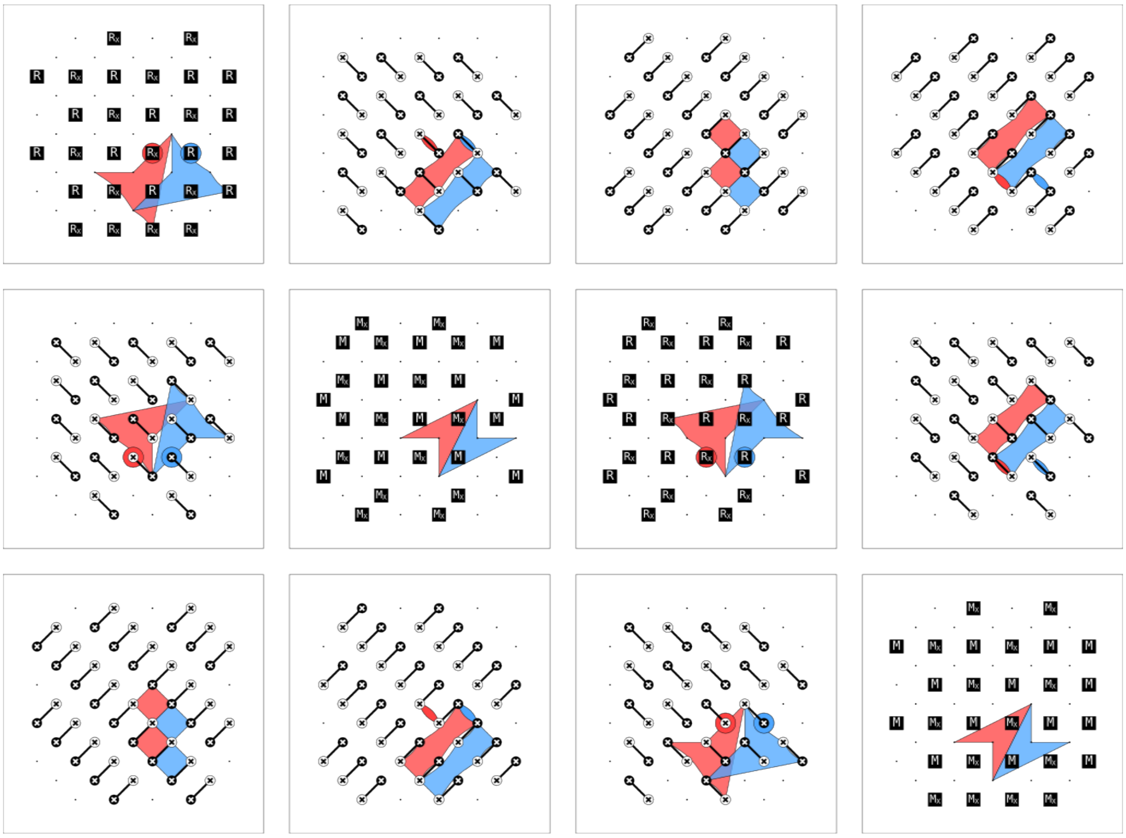

Figure 19: Circuit schedule for “3-CXSWAP-wiggle” circuits. Colored regions are elements of the instantaneous stabilizer group formed by slicing the detecting regions of a few representative detectors immediately after the displayed gate layer. Red regions are X stabilizers, blue regions are Z stabilizers, green regions are Y stabilizers, and gray regions with colored corners are mixed basis stabilizers.

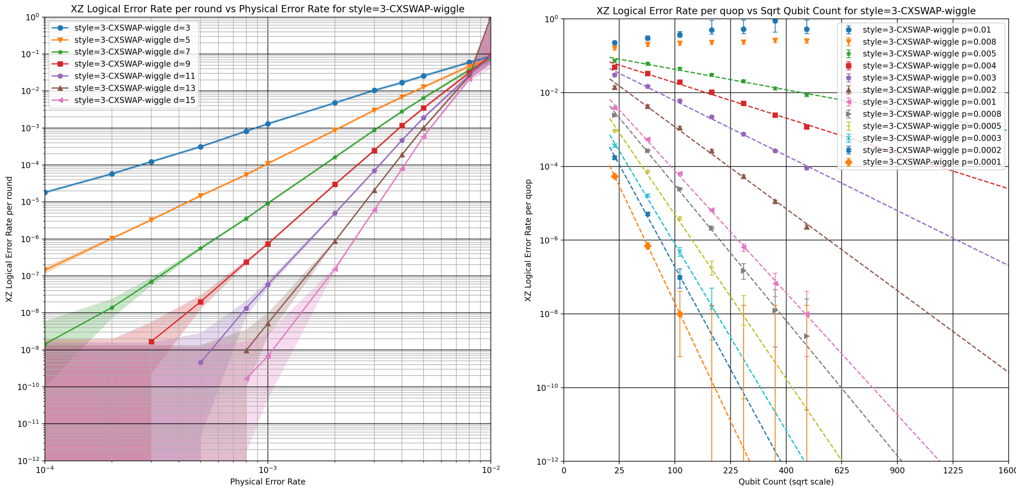


Figure 20: Threshold diagram and line fit diagram for “3-CXSWAP-wiggle” circuits. Highlighted regions cover hypotheses with likelihoods within a factor of 1000 of the maximum likelihood hypothesis. Dashed lines are least squares fits projecting the number of qubits needed to reach a target error rate.

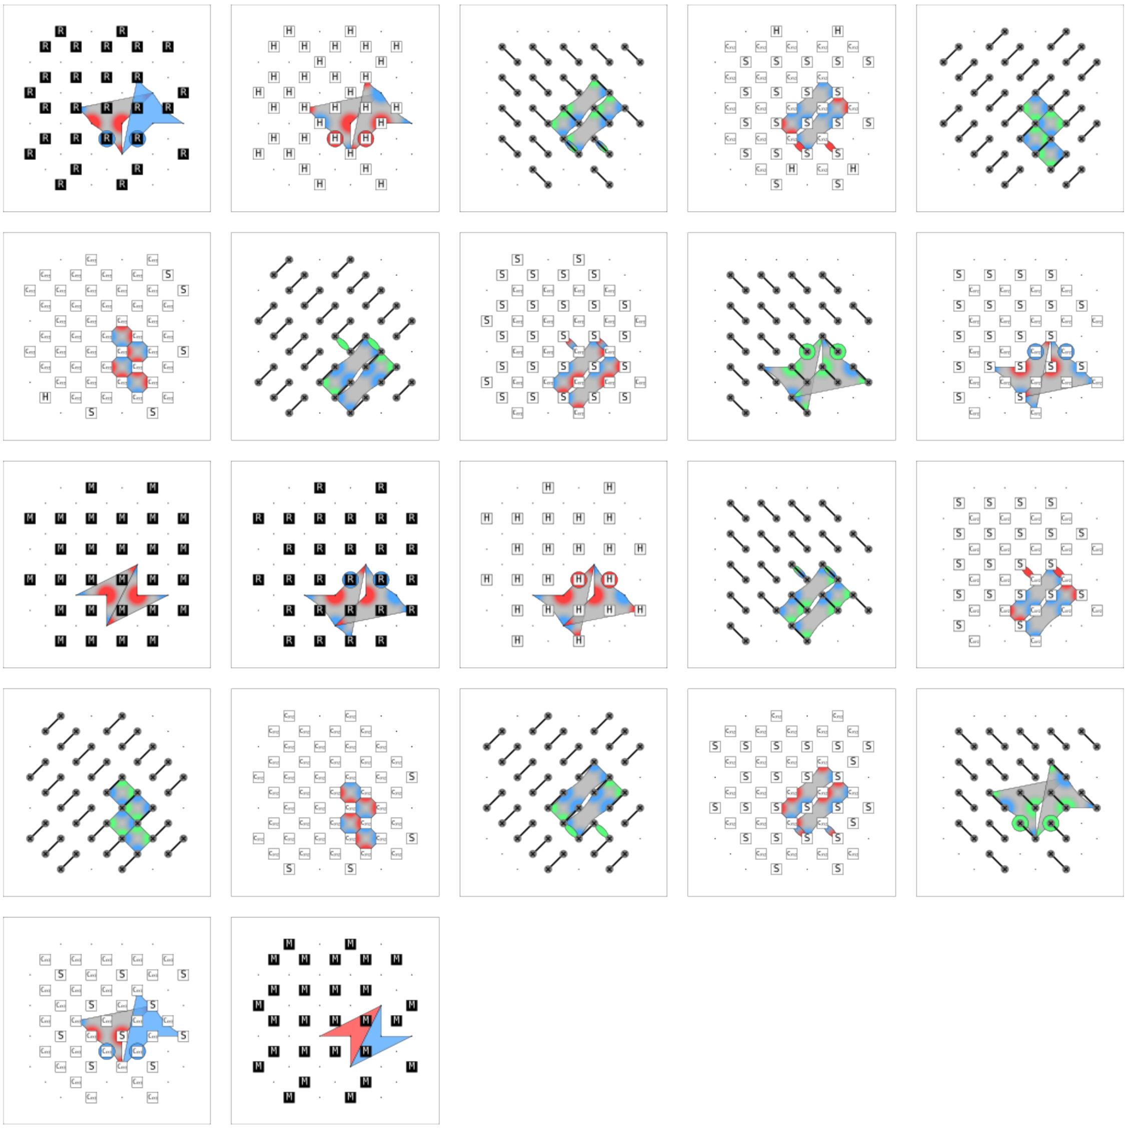

Figure 21: Circuit schedule for “3-ISWAP-wiggle” circuits. Colored regions are elements of the instantaneous stabilizer group formed by slicing the detecting regions of a few representative detectors immediately after the displayed gate layer. Red regions are X stabilizers, blue regions are Z stabilizers, green regions are Y stabilizers, and gray regions with colored corners are mixed basis stabilizers.

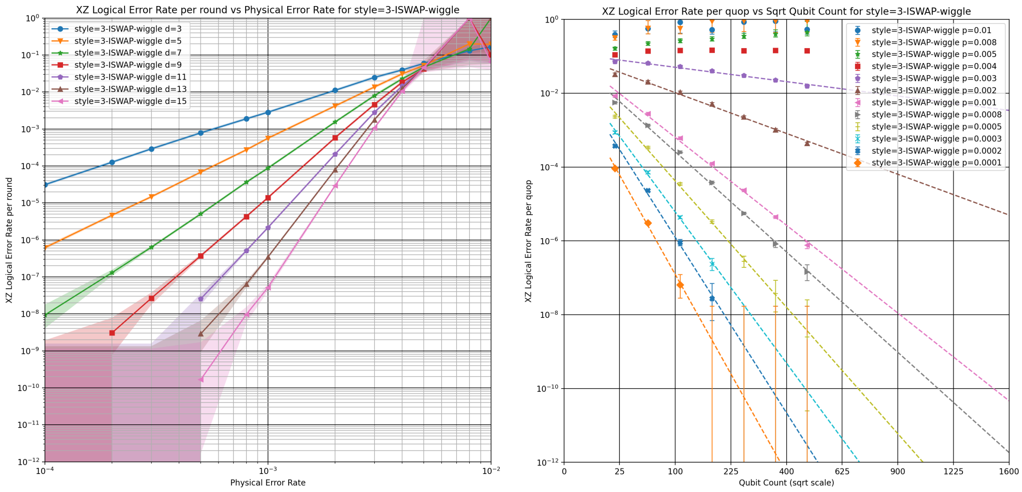


Figure 22: Threshold diagram and line fit diagram for “3-ISWAP-wiggle” circuits. Highlighted regions cover hypotheses with likelihoods within a factor of 1000 of the maximum likelihood hypothesis. Dashed lines are least squares fits projecting the number of qubits needed to reach a target error rate.

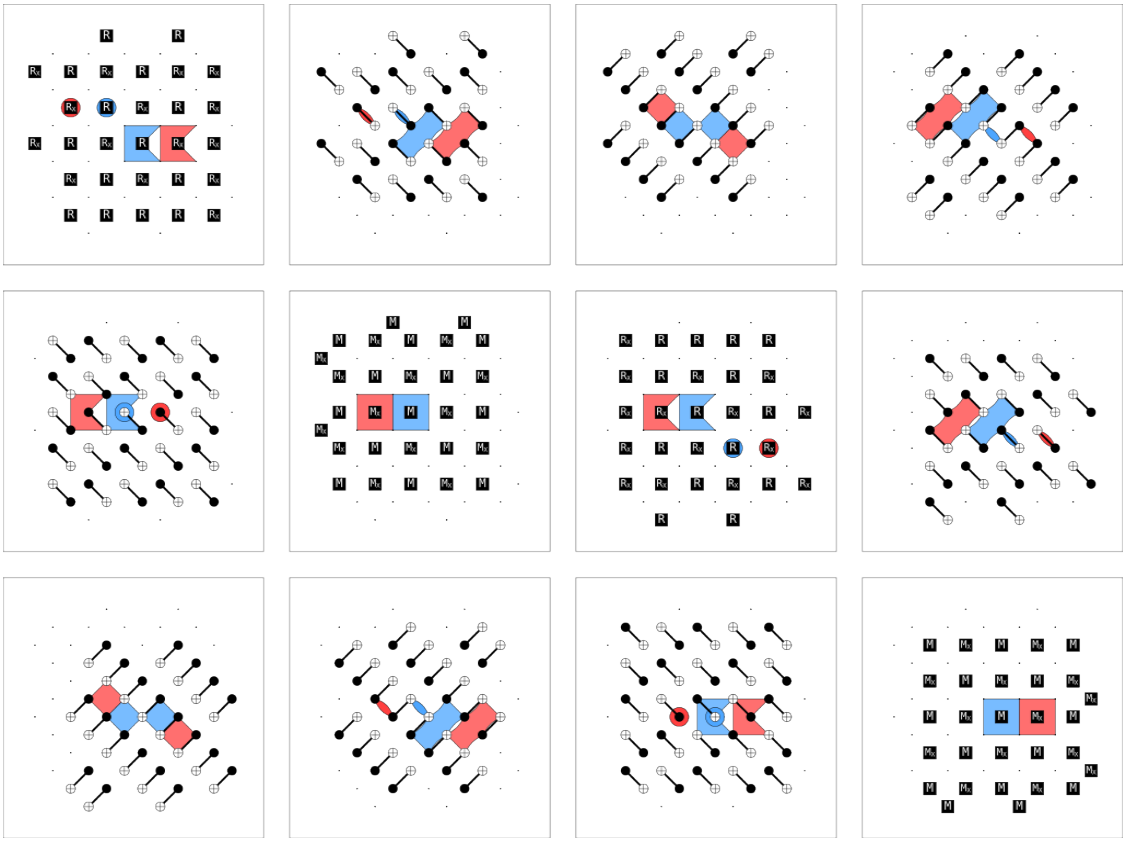

Figure 23: Circuit schedule for “WIGGLING-CX” circuits. Colored regions are elements of the instantaneous stabilizer group formed by slicing the detecting regions of a few representative detectors immediately after the displayed gate layer. Red regions are X stabilizers, blue regions are Z stabilizers, green regions are Y stabilizers, and gray regions with colored corners are mixed basis stabilizers.

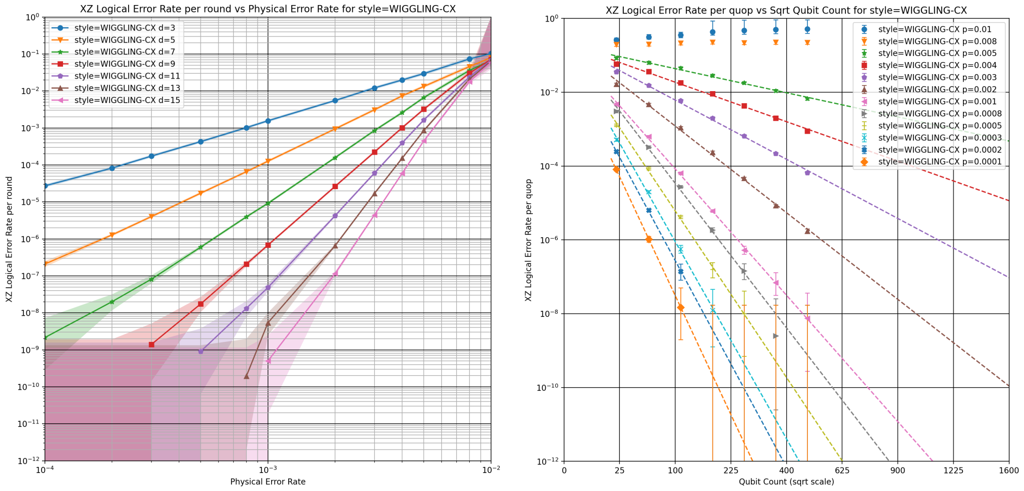


Figure 24: Threshold diagram and line fit diagram for “WIGGLING-CX” circuits. Highlighted regions cover hypotheses with likelihoods within a factor of 1000 of the maximum likelihood hypothesis. Dashed lines are least squares fits projecting the number of qubits needed to reach a target error rate.

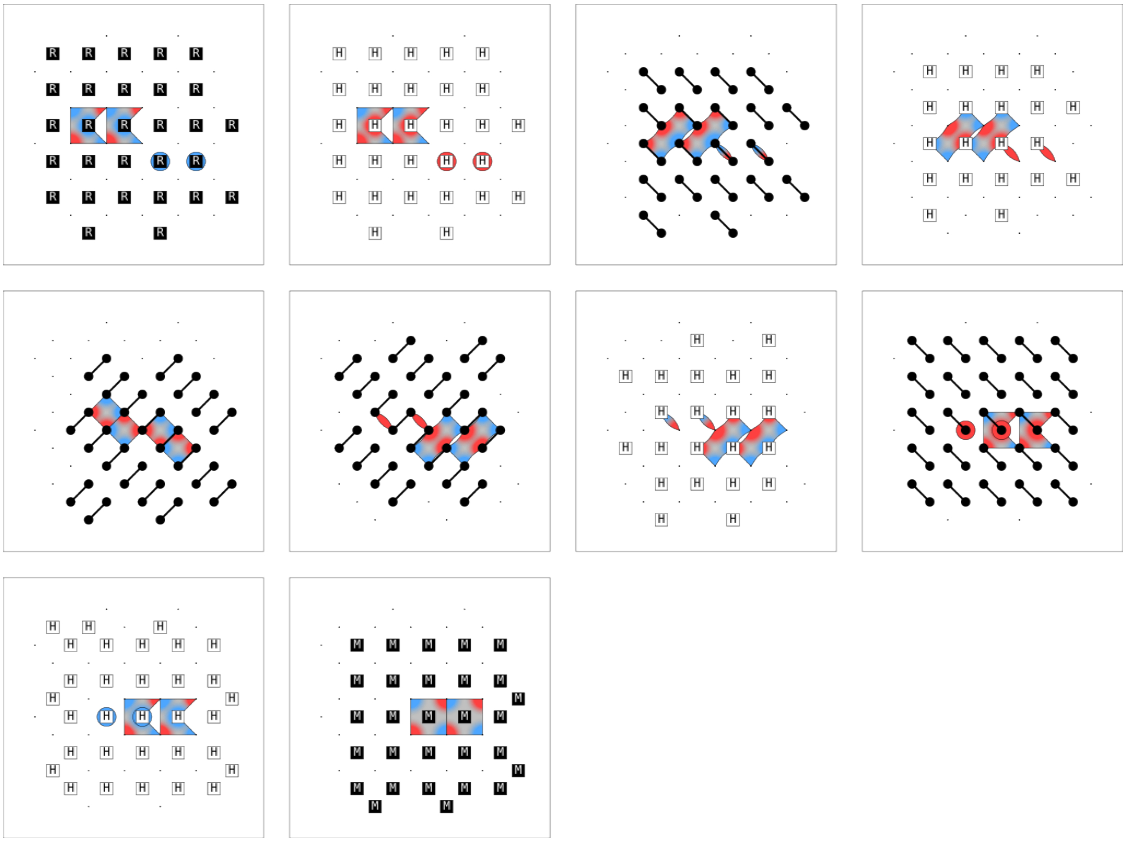

Figure 25: Circuit schedule for "WIGGLING-CZ" circuits. Colored regions are elements of the instantaneous stabilizer group formed by slicing the detecting regions of a few representative detectors immediately after the displayed gate layer. Red regions are X stabilizers, blue regions are Z stabilizers, green regions are Y stabilizers, and gray regions with colored corners are mixed basis stabilizers.

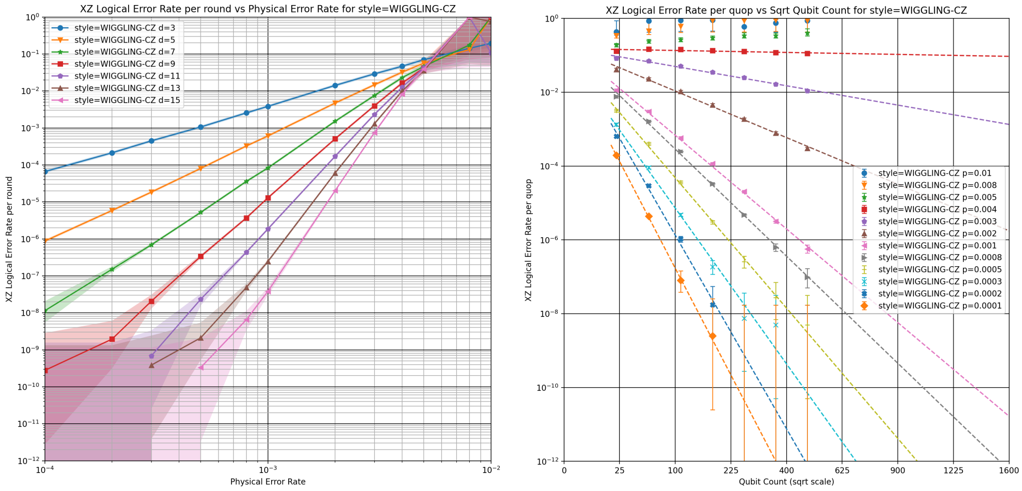


Figure 26: Threshold diagram and line fit diagram for "WIGGLING-CZ" circuits. Highlighted regions cover hypotheses with likelihoods within a factor of 1000 of the maximum likelihood hypothesis. Dashed lines are least squares fits projecting the number of qubits needed to reach a target error rate.

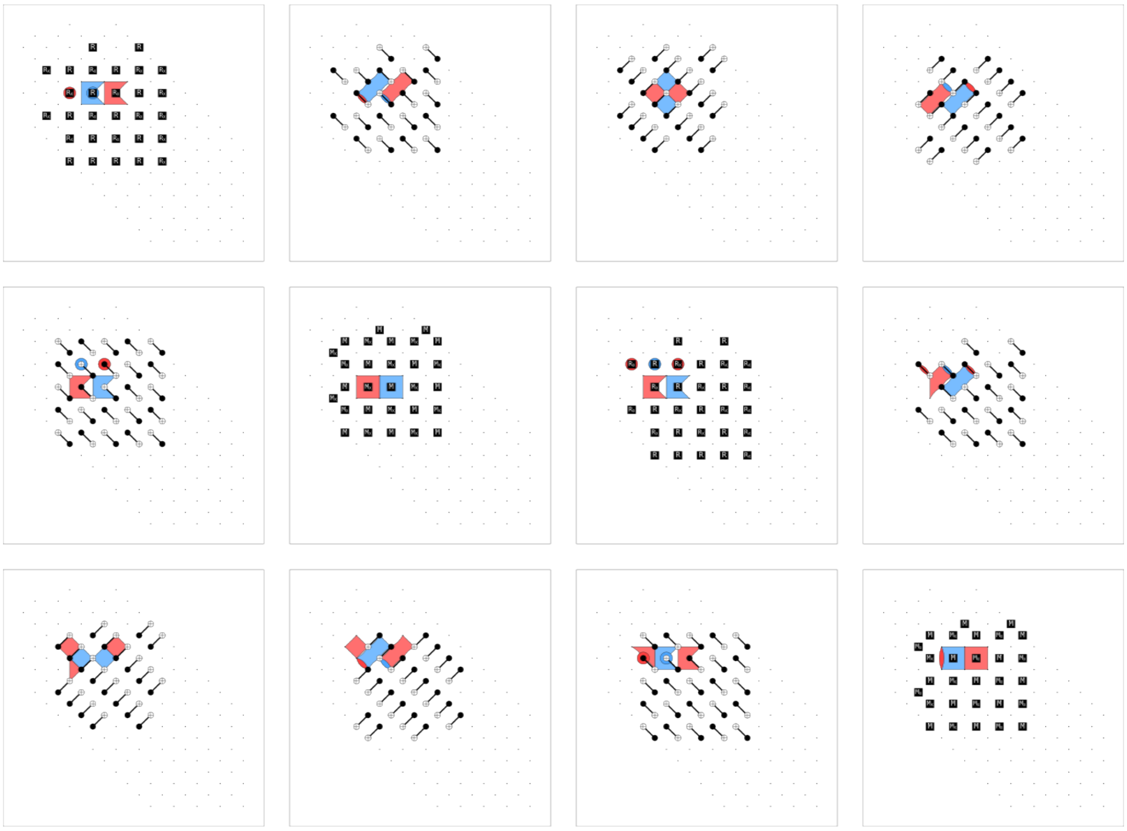

Figure 27: Circuit schedule for “GLIDING-CX” circuits. Colored regions are elements of the instantaneous stabilizer group formed by slicing the detecting regions of a few representative detectors immediately after the displayed gate layer. Red regions are X stabilizers, blue regions are Z stabilizers, green regions are Y stabilizers, and gray regions with colored corners are mixed basis stabilizers.

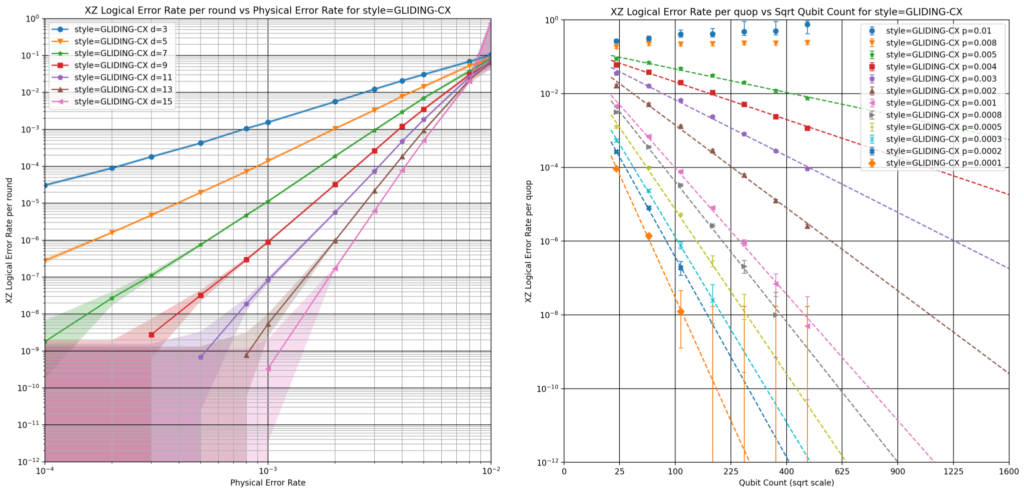


Figure 28: Threshold diagram and line fit diagram for “GLIDING-CX” circuits. Highlighted regions cover hypotheses with likelihoods within a factor of 1000 of the maximum likelihood hypothesis. Dashed lines are least squares fits projecting the number of qubits needed to reach a target error rate.

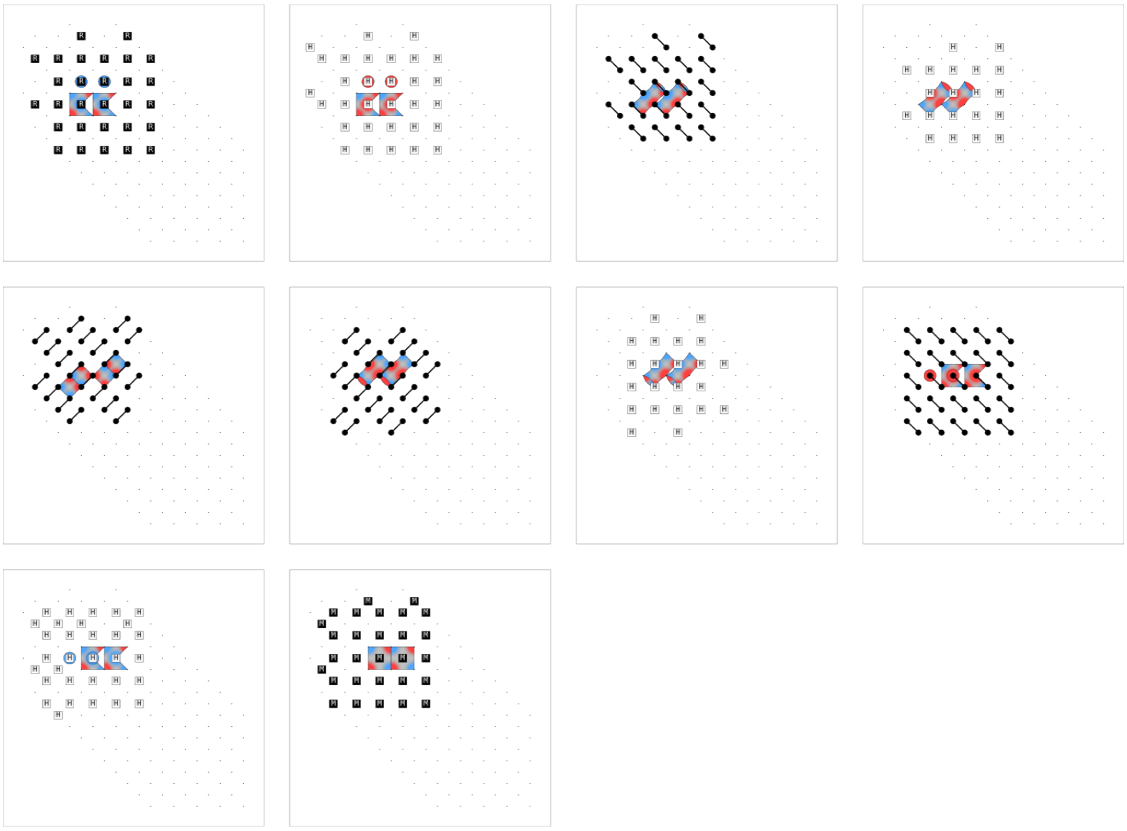

Figure 29: Circuit schedule for “GLIDING-CZ” circuits. Colored regions are elements of the instantaneous stabilizer group formed by slicing the detecting regions of a few representative detectors immediately after the displayed gate layer. Red regions are X stabilizers, blue regions are Z stabilizers, green regions are Y stabilizers, and gray regions with colored corners are mixed basis stabilizers.

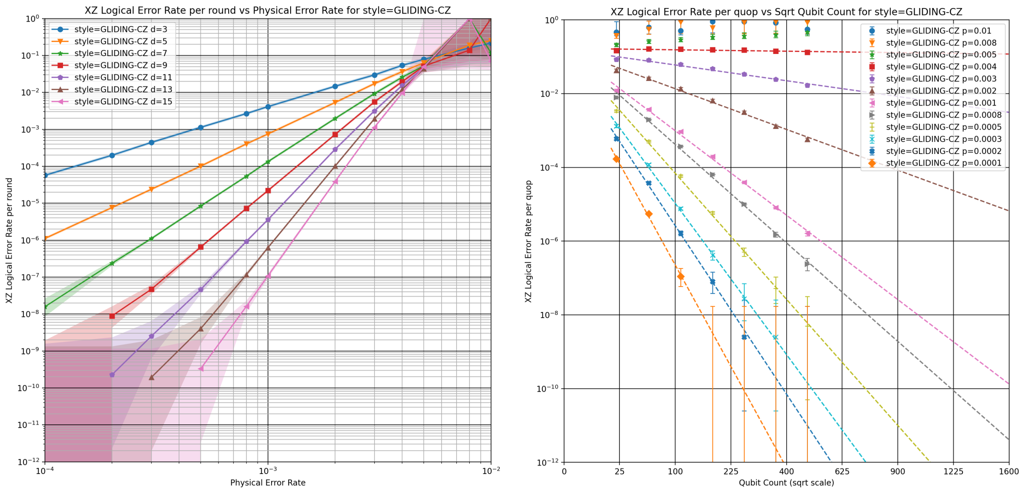


Figure 30: Threshold diagram and line fit diagram for “GLIDING-CZ” circuits. Highlighted regions cover hypotheses with likelihoods within a factor of 1000 of the maximum likelihood hypothesis. Dashed lines are least squares fits projecting the number of qubits needed to reach a target error rate.

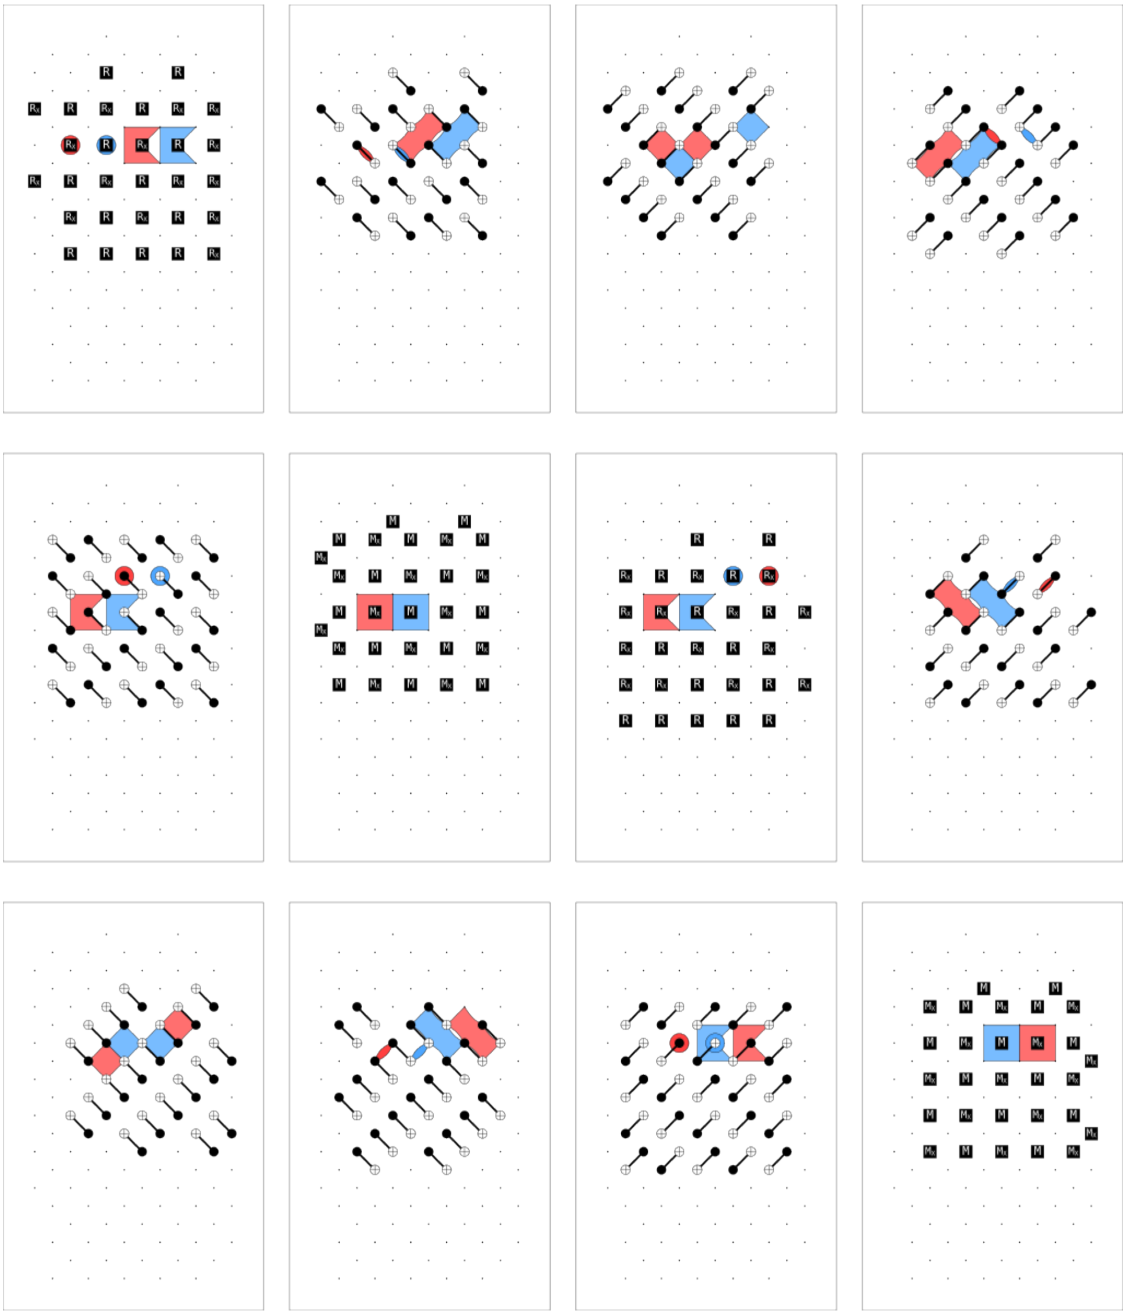

Figure 31: Circuit schedule for "SLIDING-CX" circuits. Colored regions are elements of the instantaneous stabilizer group formed by slicing the detecting regions of a few representative detectors immediately after the displayed gate layer. Red regions are X stabilizers, blue regions are Z stabilizers, green regions are Y stabilizers, and gray regions with colored corners are mixed basis stabilizers.

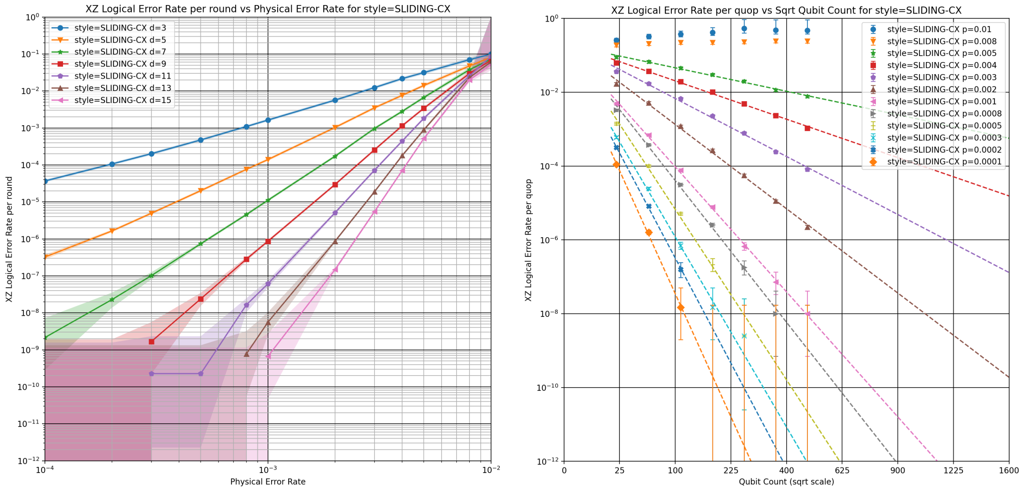


Figure 32: Threshold diagram and line fit diagram for “SLIDING-CX” circuits. Highlighted regions cover hypotheses with likelihoods within a factor of 1000 of the maximum likelihood hypothesis. Dashed lines are least squares fits projecting the number of qubits needed to reach a target error rate.

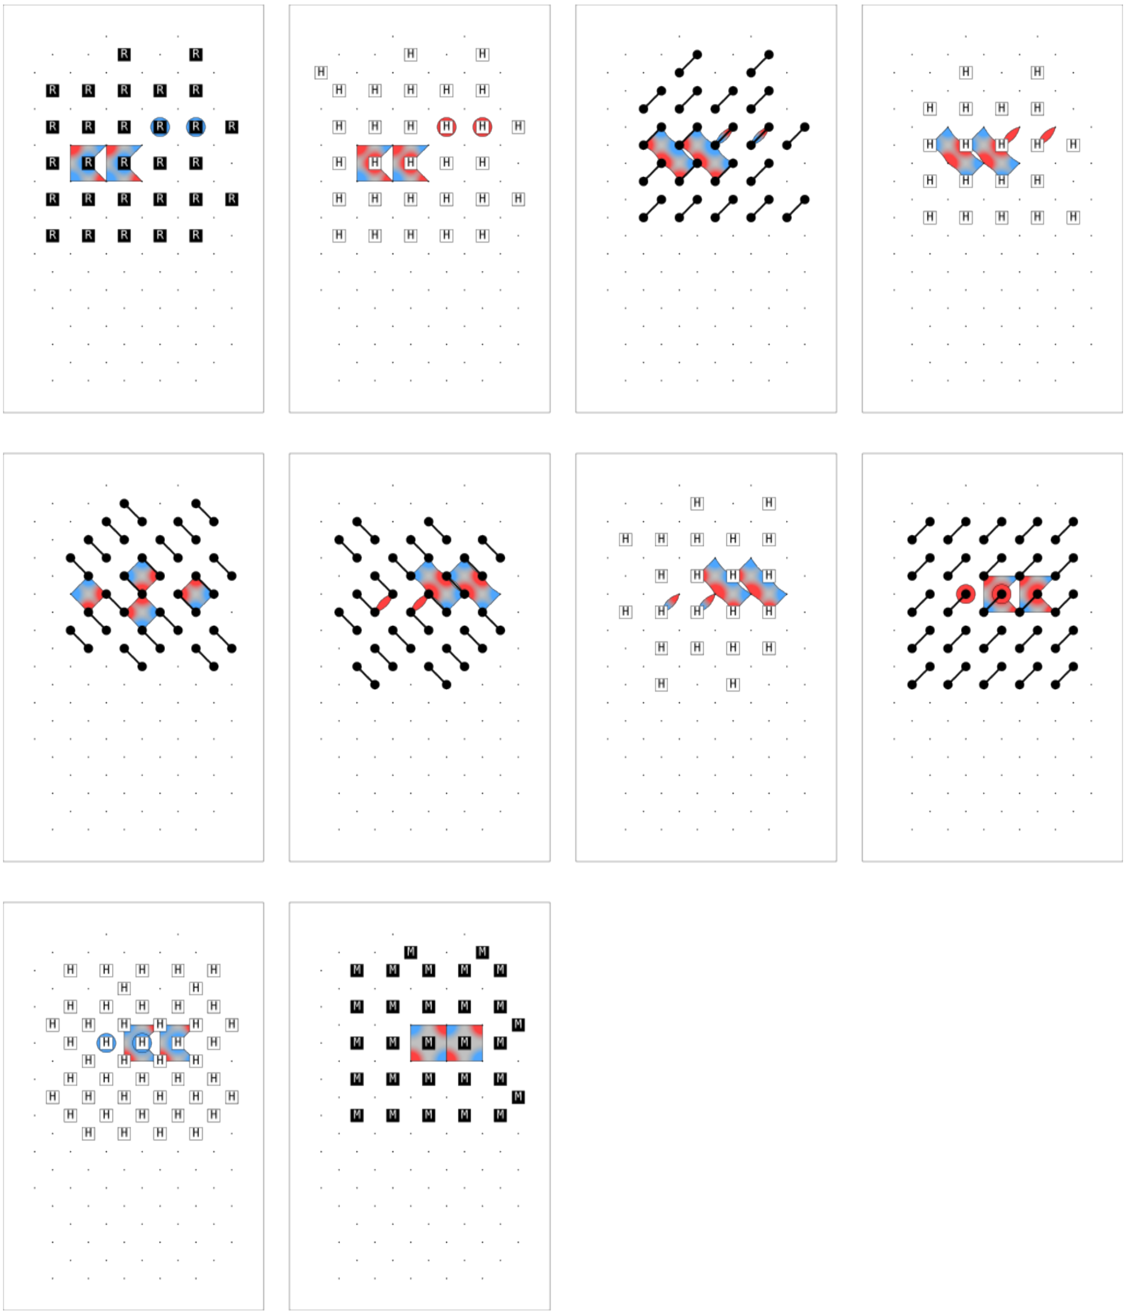

Figure 33: Circuit schedule for "SLIDING-CZ" circuits. Colored regions are elements of the instantaneous stabilizer group formed by slicing the detecting regions of a few representative detectors immediately after the displayed gate layer. Red regions are X stabilizers, blue regions are Z stabilizers, green regions are Y stabilizers, and gray regions with colored corners are mixed basis stabilizers.

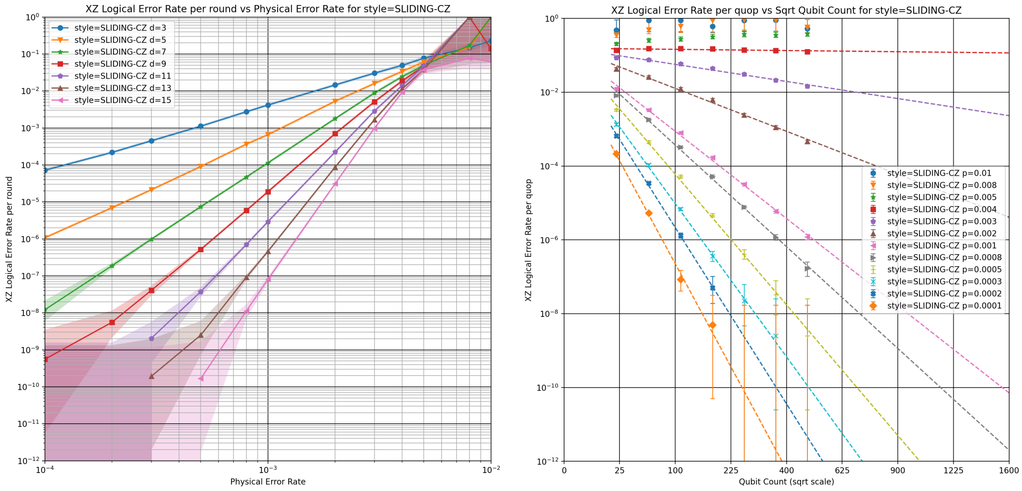


Figure 34: Threshold diagram and line fit diagram for “SLIDING-CZ” circuits. Highlighted regions cover hypotheses with likelihoods within a factor of 1000 of the maximum likelihood hypothesis. Dashed lines are least squares fits projecting the number of qubits needed to reach a target error rate.

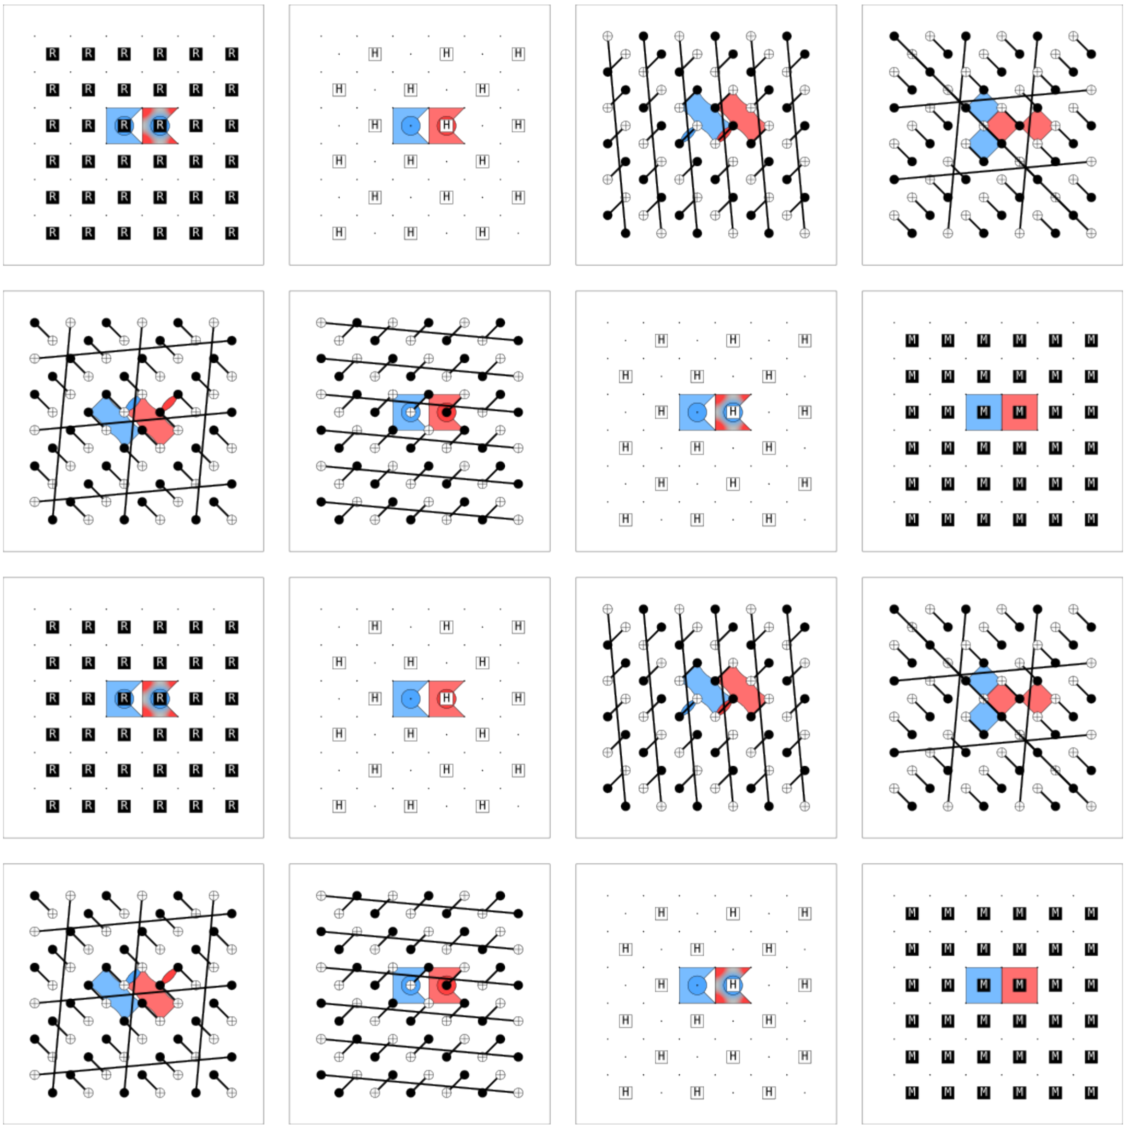

Figure 35: Circuit schedule for “TORIC-4-CX” circuits. Colored regions are elements of the instantaneous stabilizer group formed by slicing the detecting regions of a few representative detectors immediately after the displayed gate layer. Red regions are X stabilizers, blue regions are Z stabilizers, green regions are Y stabilizers, and gray regions with colored corners are mixed basis stabilizers.

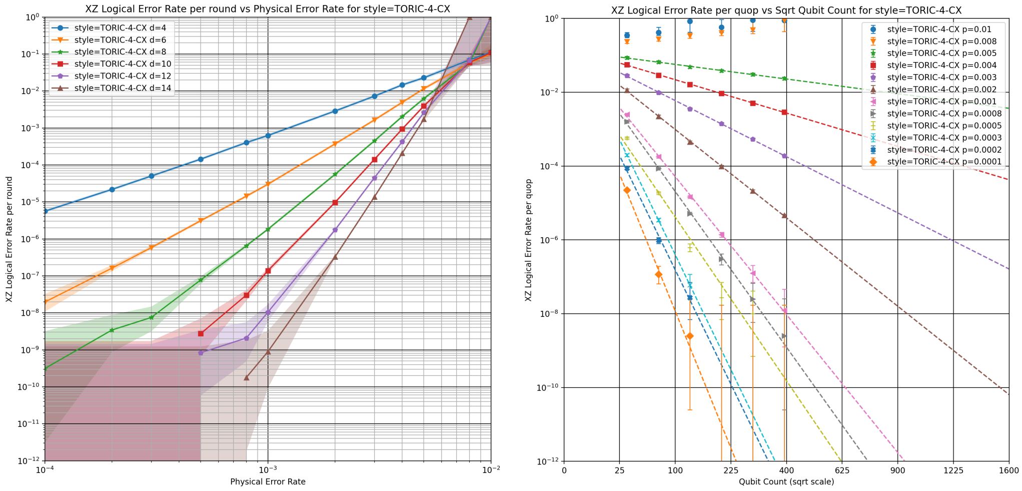


Figure 36: Threshold diagram and line fit diagram for "TORIC-4-CX" circuits. Highlighted regions cover hypotheses with likelihoods within a factor of 1000 of the maximum likelihood hypothesis. Dashed lines are least squares fits projecting the number of qubits needed to reach a target error rate.

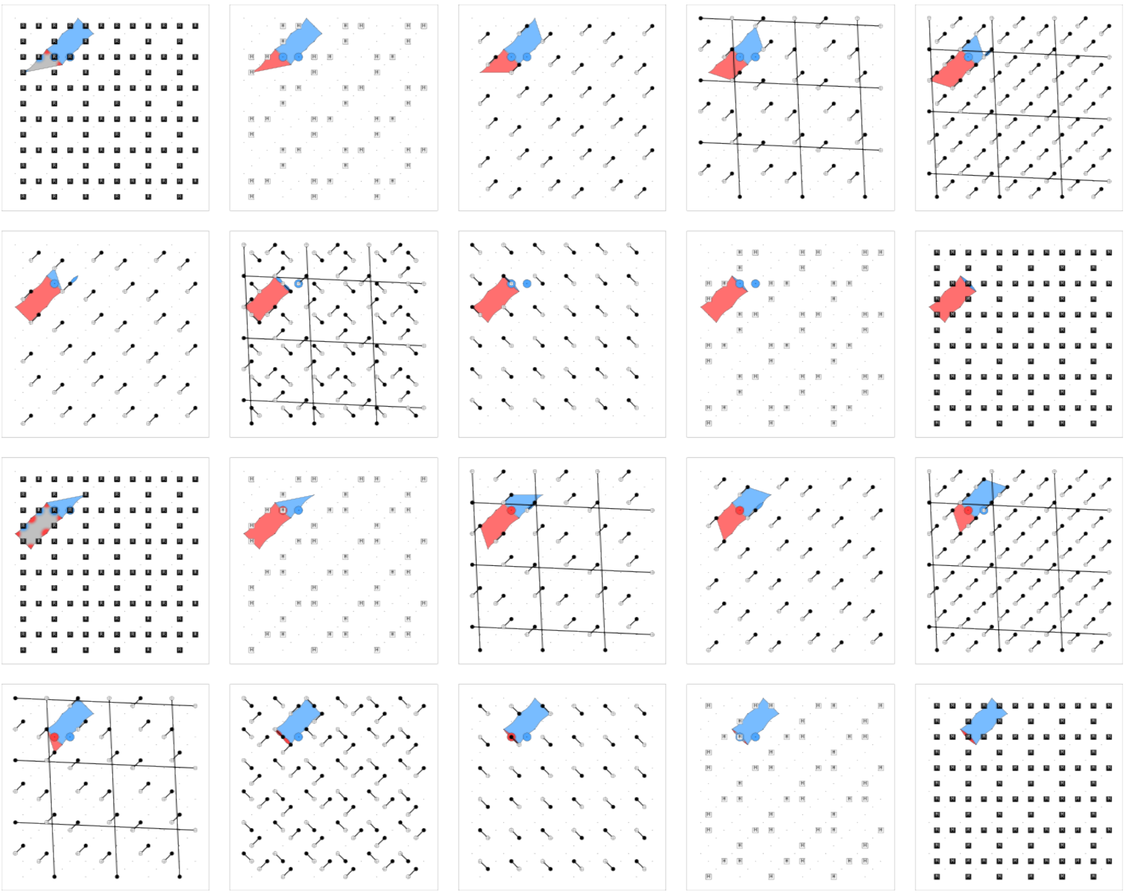

Figure 37: Circuit schedule for “TORIC-3_HEAVY-CX” circuits. Colored regions are elements of the instantaneous stabilizer group formed by slicing the detecting regions of a few representative detectors immediately after the displayed gate layer. Red regions are X stabilizers, blue regions are Z stabilizers, green regions are Y stabilizers, and gray regions with colored corners are mixed basis stabilizers.

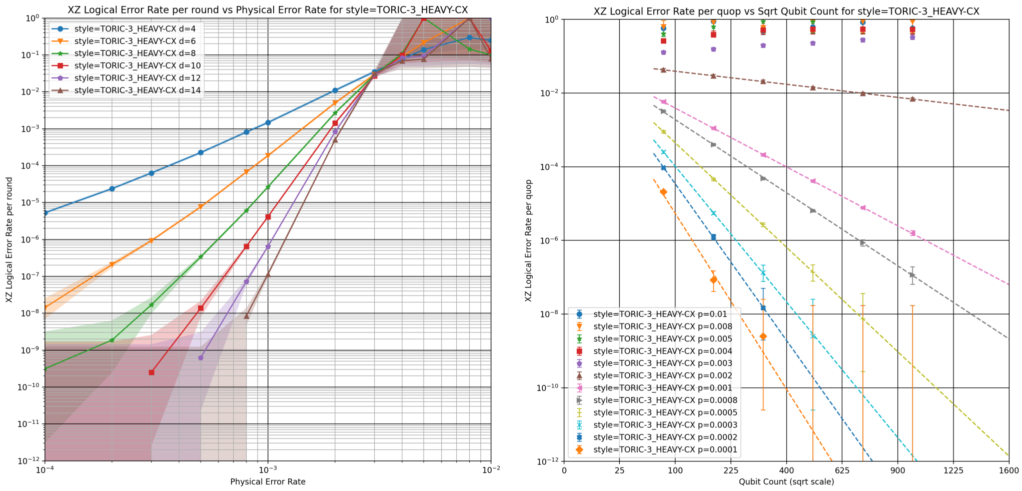


Figure 38: Threshold diagram and line fit diagram for “TORIC-3_HEAVY-CX” circuits. Highlighted regions cover hypotheses with likelihoods within a factor of 1000 of the maximum likelihood hypothesis. Dashed lines are least squares fits projecting the number of qubits needed to reach a target error rate.

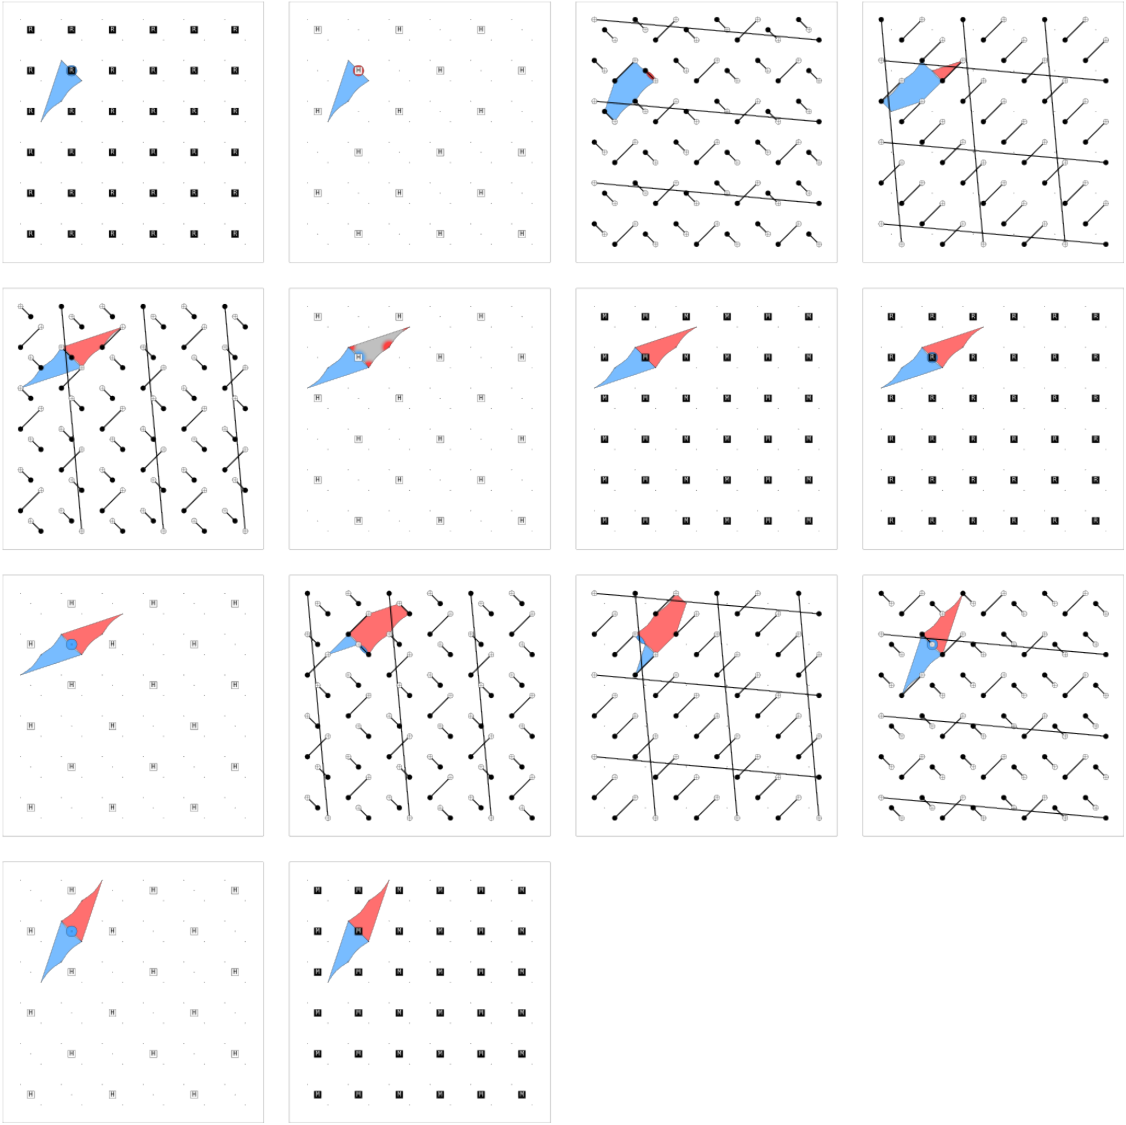

Figure 39: Circuit schedule for “TORIC-3_SEMI_HEAVY-CX” circuits. Colored regions are elements of the instantaneous stabilizer group formed by slicing the detecting regions of a few representative detectors immediately after the displayed gate layer. Red regions are X stabilizers, blue regions are Z stabilizers, green regions are Y stabilizers, and gray regions with colored corners are mixed basis stabilizers.

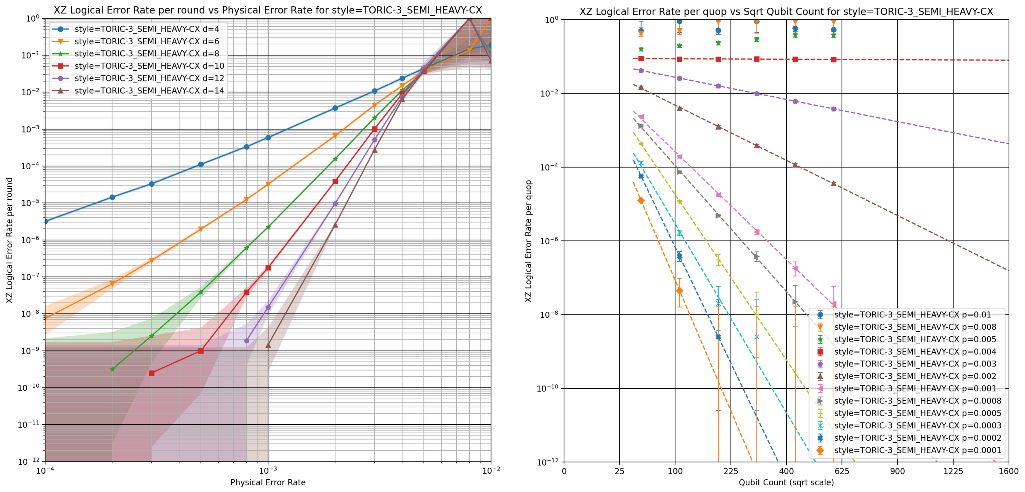


Figure 40: Threshold diagram and line fit diagram for "TORIC-3_SEMI_HEAVY-CX" circuits. Highlighted regions cover hypotheses with likelihoods within a factor of 1000 of the maximum likelihood hypothesis. Dashed lines are least squares fits projecting the number of qubits needed to reach a target error rate.

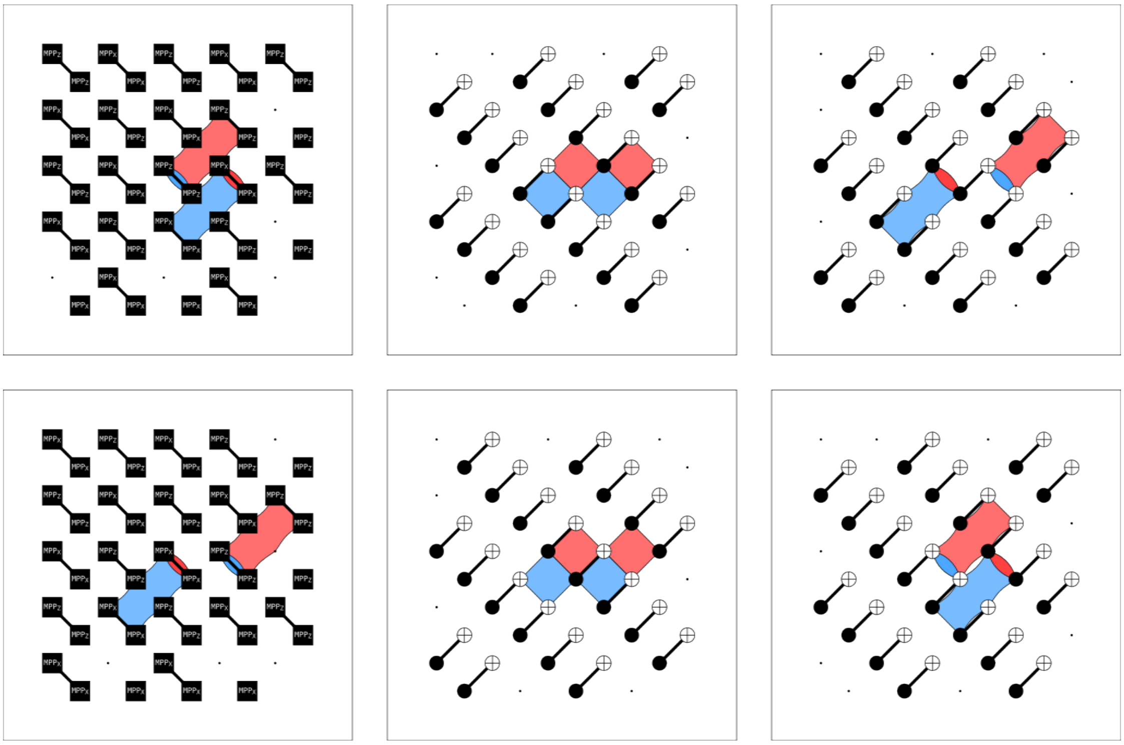

Figure 41: Circuit schedule for "3-CX_MXX_MZZ" circuits. Colored regions are elements of the instantaneous stabilizer group formed by slicing the detecting regions of a few representative detectors immediately after the displayed gate layer. Red regions are X stabilizers, blue regions are Z stabilizers, green regions are Y stabilizers, and gray regions with colored corners are mixed basis stabilizers.

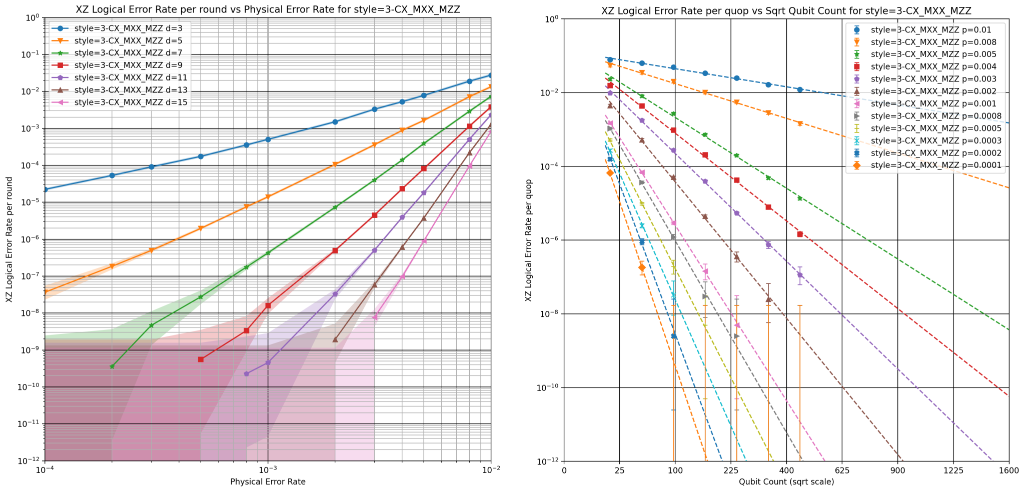


Figure 42: Threshold diagram and line fit diagram for "3-CX_MXX_MZZ" circuits. Highlighted regions cover hypotheses with likelihoods within a factor of 1000 of the maximum likelihood hypothesis. Dashed lines are least squares fits projecting the number of qubits needed to reach a target error rate.

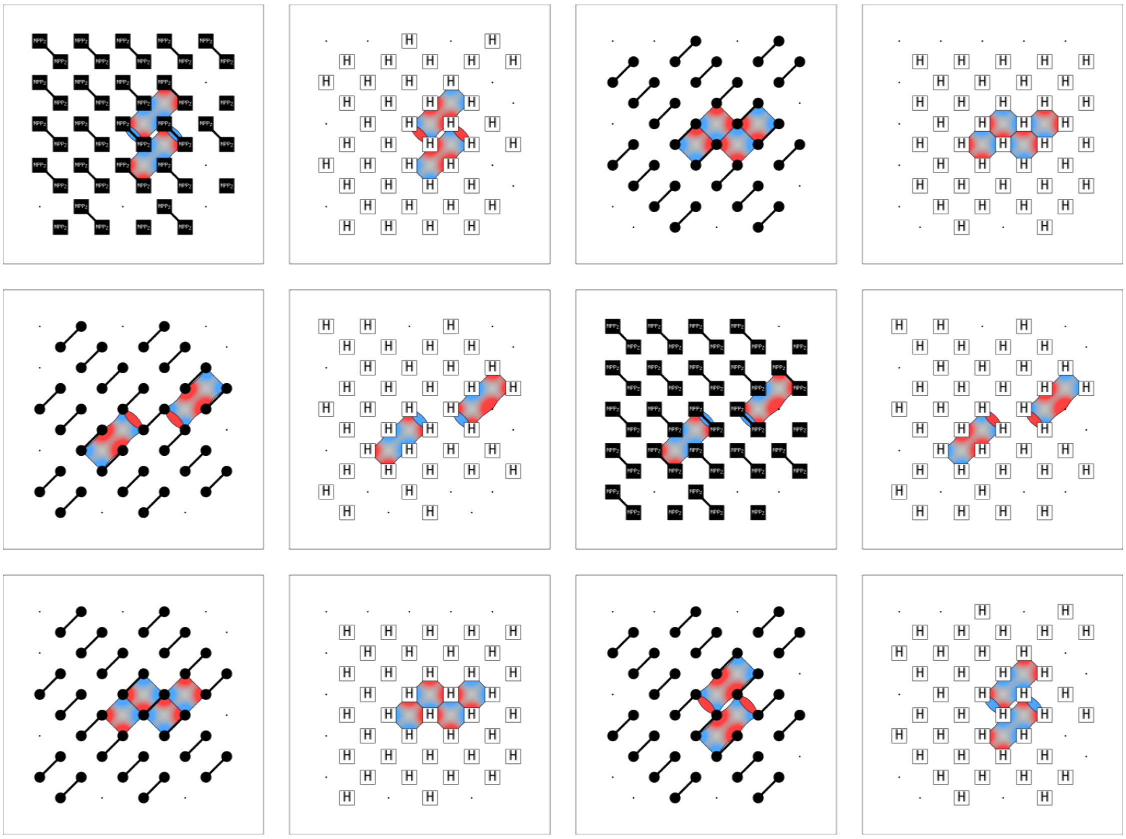

Figure 43: Circuit schedule for "3-CZ_MZZ" circuits. Colored regions are elements of the instantaneous stabilizer group formed by slicing the detecting regions of a few representative detectors immediately after the displayed gate layer. Red regions are X stabilizers, blue regions are Z stabilizers, green regions are Y stabilizers, and gray regions with colored corners are mixed basis stabilizers.

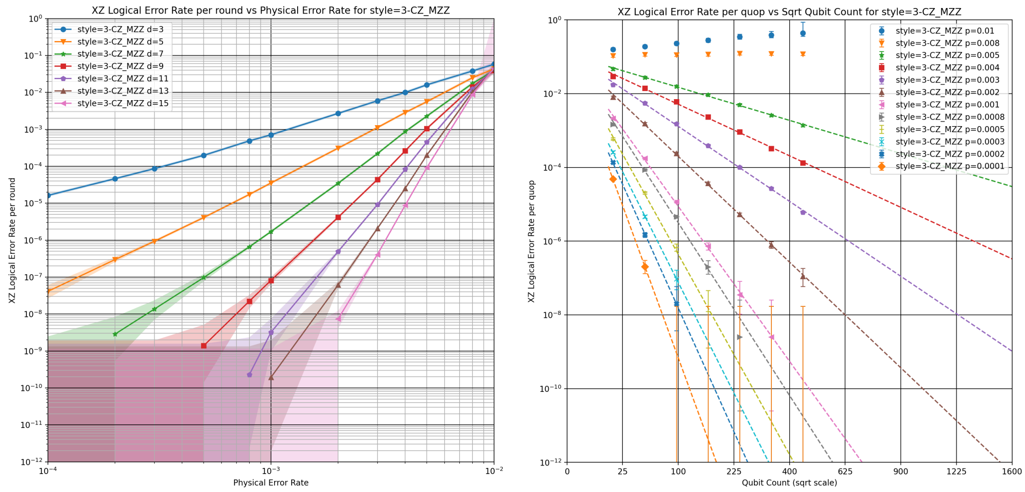


Figure 44: Threshold diagram and line fit diagram for "3-CZ_MZZ" circuits. Highlighted regions cover hypotheses with likelihoods within a factor of 1000 of the maximum likelihood hypothesis. Dashed lines are least squares fits projecting the number of qubits needed to reach a target error rate.

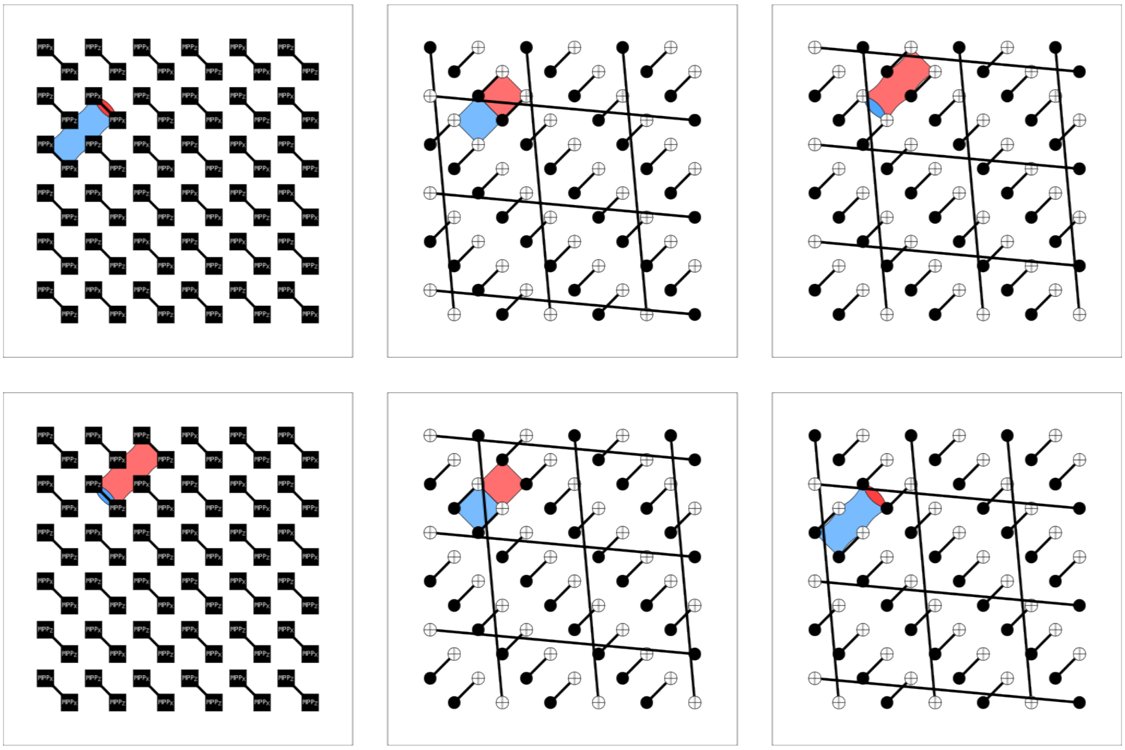

Figure 45: Circuit schedule for "TORIC-3-CX_MXX_MZZ" circuits. Colored regions are elements of the instantaneous stabilizer group formed by slicing the detecting regions of a few representative detectors immediately after the displayed gate layer. Red regions are X stabilizers, blue regions are Z stabilizers, green regions are Y stabilizers, and gray regions with colored corners are mixed basis stabilizers.

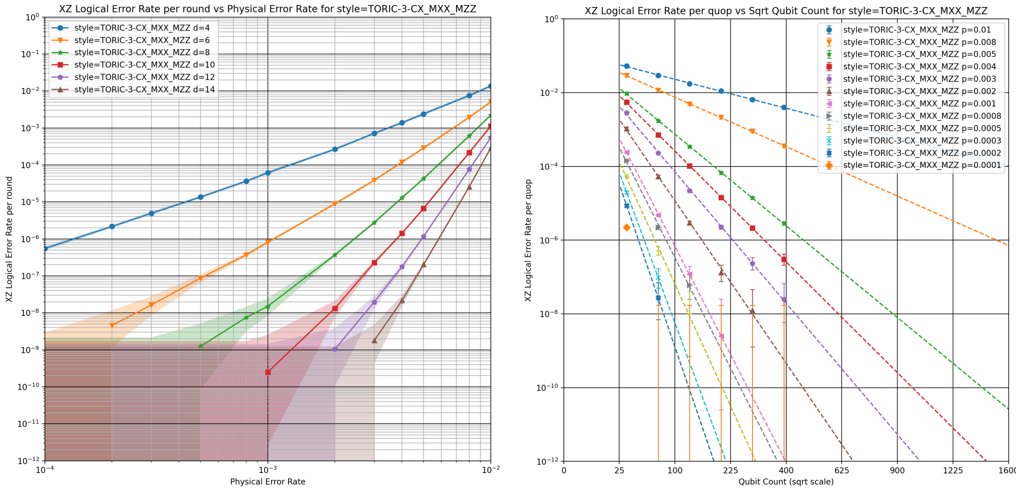


Figure 46: Threshold diagram and line fit diagram for "TORIC-3-CX_MXX_MZZ" circuits. Highlighted regions cover hypotheses with likelihoods within a factor of 1000 of the maximum likelihood hypothesis. Dashed lines are least squares fits projecting the number of qubits needed to reach a target error rate.
